# Supplementary material for: Single-Photon Switching and Entanglement of Solid-State Qubits in an Integrated Nanophotonic System
Source: arXiv:1608.05147 ancillary file (2016-08-18)
Supplement: Supplementary file 1 [file SupplementaryMaterial.pdf]

# Supplementary Material for: Single-Photon Switching and Entanglement of Solid-State Qubits in an Integrated Nanophotonic System

A. Sipahigil<sup>1,\*</sup>, R. E. Evans<sup>1,\*</sup>, D. D. Sukachev<sup>1,2,3,\*</sup>, M. J. Burek<sup>4</sup>, J. Borregaard<sup>1</sup>, M. K. Bhaskar<sup>1</sup>, C. T. Nguyen<sup>1</sup>, J. L. Pacheco<sup>5</sup>, H. A. Atikian<sup>4</sup>, C. Meuwly<sup>4</sup>, R. M. Camacho<sup>5</sup>, F. Jelezko<sup>6</sup>, E. Bielejec<sup>5</sup>, H. Park<sup>1,7</sup>, M. Lončar<sup>4</sup>, M. D. Lukin<sup>1,†</sup>

<sup>1</sup>Department of Physics, Harvard University, Cambridge, MA 02138, USA

<sup>2</sup>Russian Quantum Center, Skolkovo, Moscow 143025, Russia

<sup>3</sup>P. N. Lebedev Physical Institute of the RAS, Moscow 119991, Russia

<sup>4</sup>John A. Paulson School of Engineering and Applied Sciences,  
Harvard University, Cambridge, MA 02138, USA

<sup>5</sup>Sandia National Laboratories, Albuquerque, NM 87185, USA

<sup>6</sup>Institute for Quantum Optics, University of Ulm, 89081 Ulm, Germany

<sup>7</sup>Department of Chemistry and Chemical Biology,  
Harvard University, Cambridge, MA 02138, USA

\* These authors contributed equally to this work.

† Corresponding author. E-mail: lukin@physics.harvard.edu

## Contents

|          |                                                                                |          |
|----------|--------------------------------------------------------------------------------|----------|
| <b>1</b> | <b>Setup description</b>                                                       | <b>2</b> |
| <b>2</b> | <b>Device design, fabrication and characterization</b>                         | <b>4</b> |
| 2.1      | Cavity design . . . . .                                                        | 4        |
| 2.2      | Cavity fabrication . . . . .                                                   | 7        |
| 2.3      | Tuning the cavity resonance wavelength . . . . .                               | 8        |
| 2.4      | Cavity mode characterization using SiV centers . . . . .                       | 9        |
| 2.5      | Deterministic SiV positioning using focused Si ion beam implantation . . . . . | 10       |

|          |                                                                                       |           |
|----------|---------------------------------------------------------------------------------------|-----------|
| 2.6      | Adiabatic fiber-waveguide coupling for high-efficiency photon extraction . . .        | 11        |
| <b>3</b> | <b>Identifying single SiV centers inside nanocavities</b>                             | <b>12</b> |
| <b>4</b> | <b>SiV charge state control: high fidelity initialization and single-shot readout</b> | <b>13</b> |
| <b>5</b> | <b>Model description for a SiV center inside an optical cavity</b>                    | <b>15</b> |
| 5.1      | Three level dynamics with dissipation . . . . .                                       | 15        |
| 5.2      | System saturation response . . . . .                                                  | 16        |
| 5.3      | Calculation of intensity correlation functions . . . . .                              | 17        |
| 5.4      | Extraction of system parameters . . . . .                                             | 19        |
| 5.5      | Measured vs. expected cooperativity . . . . .                                         | 20        |
| <b>6</b> | <b>Subnatural-linewidth Raman single photons</b>                                      | <b>21</b> |
| <b>7</b> | <b>Experimental procedure for entanglement generation</b>                             | <b>23</b> |
| <b>8</b> | <b>Model description for entanglement in a two-SiV system</b>                         | <b>25</b> |
| 8.1      | Simple model . . . . .                                                                | 25        |
| 8.2      | Detailed model . . . . .                                                              | 26        |
| 8.3      | Entanglement Analysis . . . . .                                                       | 28        |
| 8.3.1    | Concurrence . . . . .                                                                 | 29        |
| 8.3.2    | Conditional fidelity estimate . . . . .                                               | 31        |
| <b>9</b> | <b>Appendix: Analytical expressions for density matrix elements</b>                   | <b>33</b> |
| 9.1      | Steady-state density matrix expressions . . . . .                                     | 33        |
| 9.2      | Coefficients in the expressions for the time-dependent density matrix elements .      | 34        |
| 9.3      | Coefficients and matrix elements for the two-SiV model . . . . .                      | 35        |

# 1 Setup description

The experiments are carried out in a confocal microscope consisting of a modified 4 K liquid helium flow probe-station (Desert Cryogenics model TTP4) and a 0.95 NA microscope objective (Nikon CFI LU Plan Apo Epi 100 $\times$ ) inside the vacuum chamber. The layout of the setup is

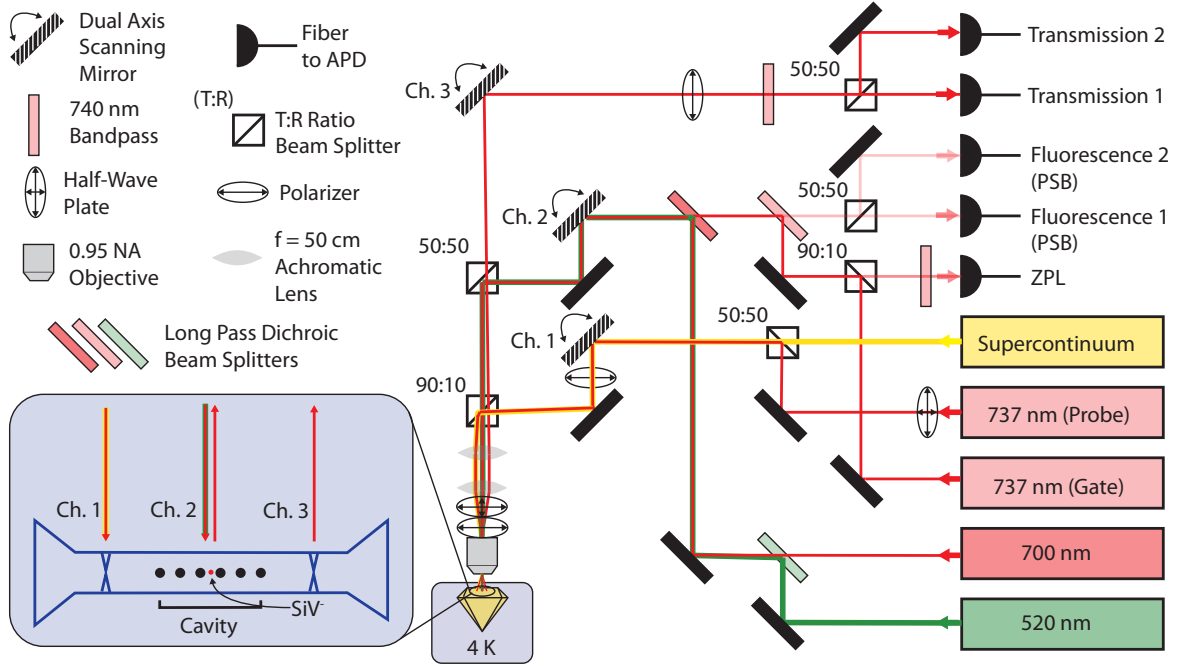

Figure S1: Optical configuration for the three-port measurements described in the main text. Each port has its own dual-axis scanning galvo mirror system (Thorlabs GVS012) labeled Ch. 1–Ch. 3. The first port, Ch. 1, is used to excite the waveguide mode and contains both a supercontinuum light source and a narrowband Ti:Saph laser used for broadband and narrowband characterization of the system response respectively. The second port, Ch. 2, is used to control the SiV (as described in Sec. 4) and monitor the SiV fluorescence scattering in the phonon-sideband (PSB). The third port, Ch. 3, is used to measure the transmission through the cavity mode. The objective and the sample are in vacuum, and the sample is cooled to 4 K. Shaded blue inset: schematic of the spatial position of the focal spots of the three channels relative to the SiV-cavity system.

shown in Fig. S1. Three ports are used to excite the system (Ch. 1), control the SiV and detect fluorescence (Ch. 2) and measure transmission (Ch. 3).

For the coarse characterization of the diamond nanocavity resonances, we excite the system with a broadband supercontinuum laser (NKT Photonics SuperKExtreme). The transmitted light is sent to a spectrometer (Horiba iHR550 with Synapse CCD and 1800 gr/mm) with a spectral resolution of 0.025 nm. To obtain high resolution spectra of the system in Fig. 1, we scanned a Ti:Sapphire laser (Probe laser: M-Squared SolsTiS-2000-PSX-XF) across the cavity and atomic resonance. For all frequency scans, the instantaneous laser frequency was monitored using a high resolution wavemeter (High Finesse WS7) with 10 MHz resolution and 50 MHz

accuracy. We used a laser noise eater (Thorlabs LCC3112H) to stabilize laser power to less than 1% during frequency scans.

We use a home-built external-cavity diode laser (Opnext Diode HL7302MG, Littrow configuration) with an electro-optical modulator (EOM: EOSPACE interferometric electro-optical amplitude modulator, model AZ-AV5-40-PFA-PFA-737 with 40 GHz bandwidth) to apply short (minimum pulse duration  $\sim 500$  ps) optical pulses for the lifetime measurements and switching experiment (Figs. 1 and 2). The interferometer of the EOM was stabilized using a lock-in amplifier (SRS model SR830) and short driving electrical pulses were generated using an arbitrary waveform generator (Tektronix AWG710, 4 GSa/s). Off-resonant excitation of the SiV was performed with 700 nm (Thorlabs LP705-SF15) and 520 nm (Thorlabs LP520-SF15) diode lasers. Single photons were counted using single-photon detectors ( $2 \times$  PicoQuant  $\tau$ -SPAD, and  $2 \times$  Excelitas SPCM-NIR) and time tagged using fast acquisition electronics (PicoQuant Hydra-Harp 400).

The waveguides described in Sec. 2 support two modes with different polarizations. In our design, the cavity mode is a transverse-electric-like (TE) mode. At the cavity resonance frequency, there is a high-transmission passband for transverse-magnetic-like (TM) modes. (Our conventions for TE and TM in this context are described in Section 2.1.) In order to only excite the relevant (TE) cavity mode, we place a polarizer immediately before the objective.

The in- and out-coupling efficiencies between free-space and waveguide modes are each of order 1% based on simulations. In order to isolate transmission from the diamond nanocavity and mitigate residual reflection from free-space optics, we use a cross-polarization scheme between the excitation (Ch. 1) and transmission (Ch. 3) channels.

## 2 Device design, fabrication and characterization

### 2.1 Cavity design

The one-dimensional diamond photonic-crystal cavity (“nanobeam cavity” hereafter) used here (based on previous designs (*1*)) consists of a diamond waveguide with a triangular cross-section perforated by a chirped 1D lattice of elliptically-shaped air holes. The unit cell of the lattice (Fig. S2A) is parameterized by the etch angle ( $\theta$ ), width ( $w$ ), lattice constant ( $a$ ) and major (transverse) and minor (longitudinal) elliptical air hole diameters ( $d_z$ ,  $d_x$ ). The unit cell etch angle (the half-angle at the bottom apex of the triangular cross-section) was fixed at  $\theta = 50^\circ$  in the design to ease fabrication.

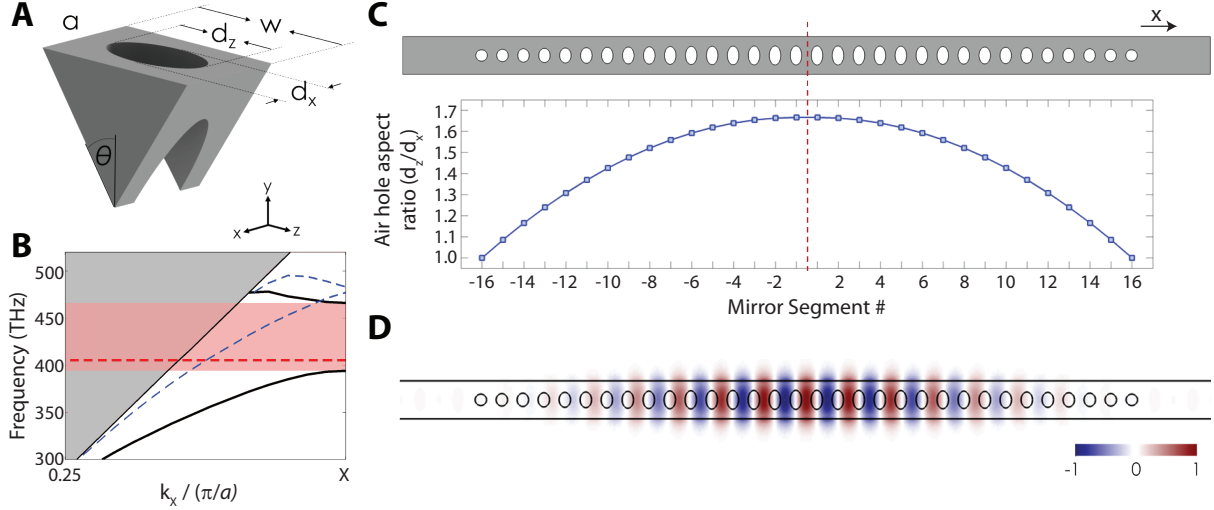

Figure S2: **(A)** Schematic of a triangular cross-section diamond unit cell parameterized by the etch angle ( $\theta$ ), width ( $w$ ), lattice constant ( $a$ ), and major and minor elliptical air hole diameters ( $d_z$ ,  $d_x$ ). **(B)** Corresponding photonic bandstructure of a nominal unit cell with  $\theta = 50^\circ$  and  $(a, w, d_z, d_x) = (260, 470, 140, 140)$  nm. The gray shaded region indicates the continuum of radiation and leaky modes that exist above the light line. Below the light line, supported transverse-electric-like (TE) and transverse-magnetic-like (TM) guided modes are indicated by solid black and dashed blue lines, respectively. A quasi-bandgap based on symmetry for the TE guided modes is indicated by the pink shaded region. The fundamental cavity resonance at  $\lambda_{TE} = 743$  nm is designated by the dashed red line. **(C)** Schematic of the 16-hole-array cavity design with the air hole aspect ratio ( $d_z/d_x$ ) plotted as a function of mirror segment number. **(D)** Normalized optical  $E_y$  field profile of the fundamental localized cavity mode of diamond nanobeam cavity design in (C).

Fig. S2B shows the photonic band structure for a nominal unit cell with  $\theta = 50^\circ$  and  $(a, w, d_z, d_x) = (260, 470, 140, 140)$  nm. Here, transverse-electric-like (TE, solid black lines) and transverse-magnetic-like (TM, dashed blue lines) guided modes give rise to symmetry based quasi-bandgaps sufficient to realize highly localized resonances. In our convention, the TE modes have odd vector symmetry with respect to reflection across the  $z = 0$  longitudinal symmetry plane of the nanobeam (see Fig. S2 for coordinate conventions). In other words, the electric field of a TE (TM) mode is mostly perpendicular (parallel) to the  $z = 0$  plane. At the center of the beam, the electric field vector of the TE modes matches the transition dipole moment of two (out of four possible) orientations of the SiV center up to a factor of  $\cos(35^\circ)$ .

We parameterized the nanobeam cavity design by the target fundamental TE cavity mode resonance wavelength in free space,  $\lambda_{TE}$ . Our final design has the following parameters: a nanobeam width  $w = 0.635 \lambda_{TE}$ , lattice constant (hole spacing)  $a = 0.349 \lambda_{TE}$  and elliptical hole minor diameter  $d_x = 0.191 \lambda_{TE}$ , with the major diameter of the elliptical hole increased quadratically, from  $d_z = d_x = 0.191 \lambda_{TE}$  at the end of the cavity, to  $d_z = 0.317 \lambda_{TE}$  at the center. This quadratically tapering major diameter is schematically displayed in Fig. S2C for a 16 hole array on each side of the cavity x-axis mirror plane. For the unit cell dimensions used to calculate the bandstructure in Fig. S2A, the fundamental TE cavity resonance is located at  $\lambda_{TE} = 743$  nm, which is designated by the dashed red line in Fig. S2B.

The total cavity loss is comprised of both radiation losses into free-space ( $Q_{rad}$ ) and coupling losses to the feeding waveguide ( $Q_{wg}$ ). For the cavity design used in the experiment, the cavity figures of merit generated from FDTD simulations are the cavity mode volume ( $V = 1.8 (\lambda_{TE}/n)^3$  with  $n = 2.4$ ) and the partial optical Q-factors ( $Q_{rad} \approx 320000$ ,  $Q_{wg} \approx 10000$ ). From the partial optical Q-factors, the total cavity loss ( $Q_{tot}$ ) is given by the relation  $Q_{tot} = (Q_{rad}^{-1} + Q_{wg}^{-1})^{-1} \approx 10000$ . Additionally, the predicted on-resonance transmission of the fundamental cavity mode was calculated by the relation:  $T = Q_{tot}^2 / Q_{wg}^2 \approx 94\%$ . It is important for this transmission to be high because it is directly proportional the number of photons we are able to measure experimentally.

In order to estimate the transmission of the cavities used in the experiment, the cavity transmission was normalized to transmission through a diamond waveguide (no holes) with identical in- and out-coupling structures. Using this approach, we found that the cavity transmission on resonance was  $\geq 85\%$  of the waveguide transmission.

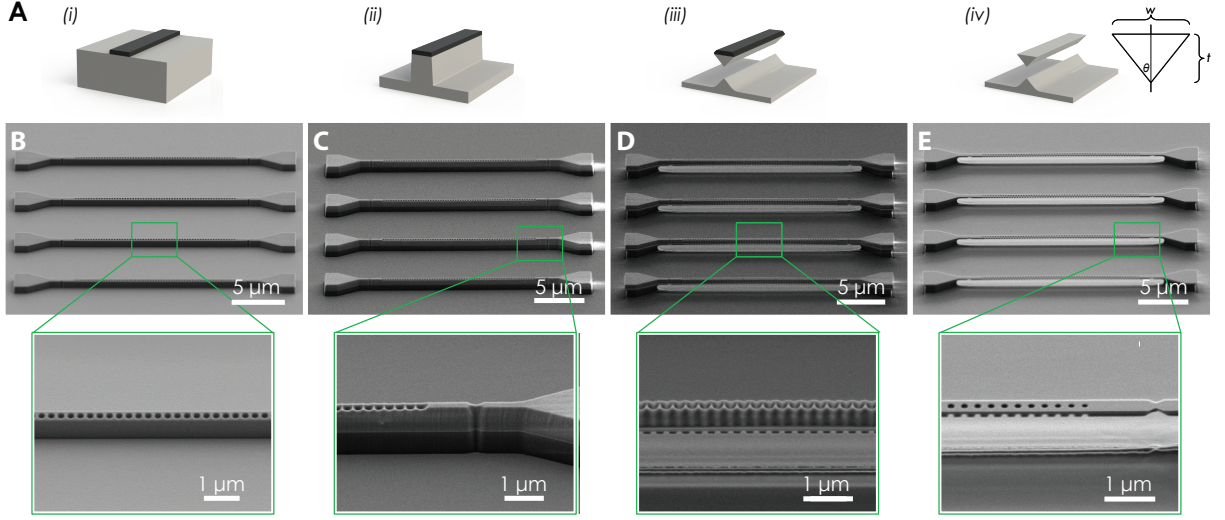

Figure S3: **(A)** Illustration of the angled-etching technique used to fabricate free-standing optical nanocavity structures in bulk single-crystal diamond. Angled-etching fabrication steps with corresponding SEM images: **(i)** define an etch mask on substrate via standard fabrication techniques (panel **(B)**), **(ii)** transfer etch mask pattern into the substrate by top-down plasma etching (panel **(C)**), **(iii)** employ angled-etching to realize suspended nanobeam structures (panel **(D)**), **(iv)** remove residual etch mask (panel **(E)**). All SEM images taken at a stage tilt of  $60^\circ$ .

## 2.2 Cavity fabrication

Electronic grade,  $\langle 100 \rangle$ -normal oriented, single-crystal diamond substrates (CVD grown,  $< 5$  ppb [N], Element Six), were first polished to a surface roughness  $< 5$  nm RMS, followed by an acid treatment (“tri-acid clean” hereafter) in a boiling mixture consisting of equal parts conc. sulfuric acid, conc. nitric acid, and 70% (aqueous) perchloric acid. Prior to device fabrication, approximately the top six microns of the diamond surface were removed in a standard inductively-coupled-plasma reactive-ion etcher (ICP-RIE, Unaxis Shuttleline). This pre-fabrication etch consisted of an  $\text{Ar}/\text{Cl}_2$  etch (30 minutes, 400 W ICP power, 250 W RF power, 25 sccm Ar flow rate, 40 sccm  $\text{Cl}_2$  flow rate, 8 mTorr chamber pressure) followed by an  $\text{O}_2$  etch (30 minutes, 700 W ICP power, 100 W RF power, 50 sccm  $\text{O}_2$  flow rate, 10 mTorr chamber pressure). This pre-fabrication etch removes polishing-induced mechanical strain near the top surface of the diamond and reduces the final surface roughness of the diamond substrate to  $< 1$  nm RMS (confirmed by AFM (2)).

Our nanofabrication procedure is outlined schematically in Fig. S3. First, a silica etch mask was patterned on the prepared diamond substrates using electron-beam lithography on a 650 nm

spin-coated layer of 83% hydrogen silsesquioxane (HSQ, FOX-16 from Dow Corning) negative resist in methyl isobutyl ketone (MIBK). Exposed HSQ was developed in tetramethylammonium hydroxide (TMAH, 25% diluted aqueous solution) to yield the final mask used for etching (Fig. S3B).

We then performed a conventional top-down anisotropic plasma etch (Unaxis Shuttleline ICP-RIE, 700 W ICP power, 100 W RF power, 50 sccm O<sub>2</sub> flow rate, 2 sccm Ar flow rate, 10 mTorr chamber pressure) to first transfer the silica etch mask pattern into the diamond to a depth of approximately 600 nm (Fig. S3C). We then etched the sample at an angle using the same ICP-RIE parameters as the initial top down etch, but instead housing the sample inside a macroscopic aluminum Faraday cage (3, 4) to direct the plasma ions to the substrate surface at the intended angle (Fig. S3D). Finally, the remaining etch mask was removed in concentrated hydrofluoric acid, followed by 1 : 3 hydrogen peroxide : conc. sulfuric acid (“piranha”) solution leaving freestanding diamond nanocavities (Fig. S3E).

After the cavities are fabricated, SiV centers are created by targeted implantation using a focused ion beam. This technique will be described in Section 2.5. Implantation is followed by a tri-acid clean and a three-stage ultra-high-vacuum (maximum pressure  $5 \times 10^{-9}$  Torr) anneal at 400°C (3°C per minute ramp, 8 hour dwell time), 800°C (1°C per minute ramp, 8 hour dwell time), and 1200°C (1°C per minute ramp, 4 hour dwell time). This annealing introduces a small amount of graphitic carbon on the surface of the sample. The tri-acid clean is repeated after annealing to remove this carbon. We do not perform a low temperature oxygen anneal. This procedure is described in more detail elsewhere (5, 6).

## 2.3 Tuning the cavity resonance wavelength

Fabrication imperfections usually result in cavity resonances that are typically of order 10 nm away from the desired resonance position. Moreover, cooling the sample to 4K introduces additional irreproducible shifts due to thermal contraction of diamond and condensation of residual gas onto the sample surface. Thus, it is highly desirable to have a method to tune the resonance frequency of the cavity *in situ* during the course of our experiment.

To accomplish this goal, we deliberately introduce a controlled amount of inert gas into the chamber (7). This gas freezes on the surface of the sample, increasing the local refractive index and shifting the resonance frequency of the cavity to longer wavelengths. Using this technique, we can tune the cavity resonance by more than 20 nm with no deterioration of the cavity quality factor.

Thermal desorption of the tuning gas provides a simple technique to reverse the tuning. Either the sample can be heated up locally using an intense laser field, and/or the whole sample can be heated using a resistive heater mounted on the sample stage. The tuning procedure is very robust and was implemented on the same diamond nanophotonic device many times over several months. For our experiment, we use carbon dioxide as the tuning gas which does not desorb under typical experimental conditions but can be desorbed deliberately using the above methods.

## 2.4 Cavity mode characterization using SiV centers

We estimate the mode volume of the nanobeam cavity experimentally by probing the local photonic density of states, which is in turn measured via the spontaneous emission rate of SiV centers into the cavity mode. To implement this novel technique, we use a sample with a similar cavity design but a very high density of SiV centers created by uniform high-density ion implantation (implantation flux  $3 \times 10^{11} \text{ cm}^{-2}$ , implantation energy 150 keV, performed by Innovion corporation). We then tune the cavity as described in the previous section until the ensemble of SiV centers is on resonance with the fundamental mode of the cavity. Next, we excite the SiV centers in the cavity by scanning over the entire nanostructure with an off-resonant excitation laser at 700 nm (Ch. 2 in Fig. S1 and S4). We measure the fluorescence into the cavity mode via the outcoupling notch at the end of the cavity (Ch. 3). To produce a one-dimensional plot of the mode density along the beam, we integrate along the direction ( $z$ ) orthogonal to the beam. We then repeat this procedure for the second-order cavity mode by tuning the mode into resonance with the SiV ensemble.

Figure S4: (A) Scanning electron micrograph of nanophotonic crystal cavity and (B) simulated energy density profile of the cavity mode. (C) Experimentally measured energy density profile for the cavity mode in part B. Photons are detected in the waveguide mode (Ch. 3) as the excitation laser (Ch. 2) is spatially scanned across the nanocavity.

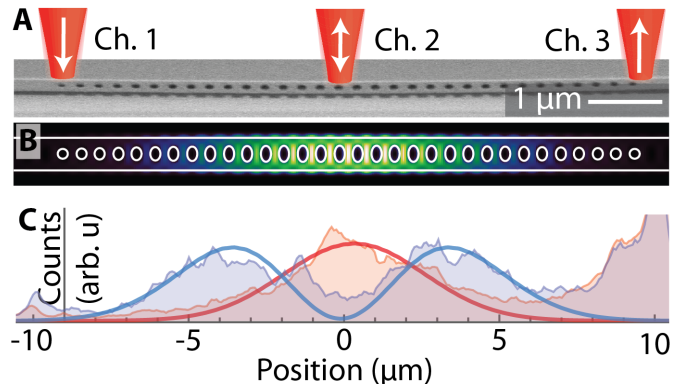

Figure S4C shows this integrated line cut superimposed with the same integrated line cut taken from our FDTD simulations (see Section 2.1) where the horizontal axis has been scaled

by a fitted parameter to estimate the agreement between simulations and experiment. We assume that the transverse mode profile is given by our simulated value since that mode profile is determined primarily by the size and refractive index of the beam which are well controlled. Before fitting, the simulated data has been convolved with a Gaussian point-spread function ( $2\sigma \approx 600$  nm) with width extracted from an image of a single emitter.

We find that the measured mode volume is 35% larger for the first mode and 46% larger for the second mode than predicted by our simulations. Under the assumption that this scaling is similar for the devices used in the main text, we estimate an experimental mode volume for the first mode of  $V \sim 2.5 (\lambda/n)^3$  (here,  $n = 2.4$ ). Discrepancies in the mode volume can result from fabrication imperfections which can reduce longitudinal confinement. This mechanism is plausible since we have observed lower quality factors than predicted in our simulations (see Section 2.1).

## 2.5 Deterministic SiV positioning using focused Si ion beam implantation

SiV centers were introduced at the center of the diamond nanocavities by targeted implantation using Sandia National Lab’s nanoImplanter, a custom focused-ion-beam system made by the A&D Corporation (Tokyo). This instrument employs a 100 kV accelerating potential, an  $E \times B$  mass velocity filter with  $m/\Delta m = 60$ , a laser interferometry controlled stage and a Raith Elphy Plus pattern generator. A AuSiSb liquid metal alloy is used to generate the  $\text{Si}^+$  ion beam. We controlled the ion fluence with a combination of beam current and dwell time at each targeted implantation site. The implantation position was aligned to  $<1$  nm.

This combination of controlled ion fluence, energy and positioning allows for precise control over the number, depth and lateral position of SiV centers inside the nanophotonic structure. The number of implanted ions obeys a Poisson distribution; the error in the number of implanted ions scales as the square root of the average number of implanted ions. The expected positioning error is dominated by the ion spot size (40 nm). The range (depth) of the ions is predicted to be 68 nm with a  $\pm 13$  nm straggle (from SRIM simulations (8)). The positioning error is about a factor of two smaller than the relevant cavity mode dimensions: the mode oscillates at about 100 nm peak-to-peak in the longitudinal direction and has a similar extent in the transverse directions.

Using this approach, we chose an intended dose of between 10 to 500 ions (equivalent fluence  $8 \times 10^{11}$  to  $4 \times 10^{13}$  ions/cm<sup>2</sup>) for different nanocavities on the diamond sample. The nanocavity used in the experiment was implanted with 350  $\text{Si}^+$  ions and contains more than

5 SiV centers (Fig. S5) after high temperature annealing. These measurements demonstrate greater than 1.5% conversion yield from  $\text{Si}^+$  ions to SiV centers, comparable to what has been realized in the bulk (6). The yield of conversion from  $\text{Si}^+$  ions to SiV centers is limited by the vacancy density in the diamond crystal. Electron irradiation has been shown to improve the SiV creation yield by more than an order of magnitude (9) and could be used to enable operation with fewer number of implanted ions, reduced damage to the crystal and reduced inhomogeneous distribution.

## 2.6 Adiabatic fiber-waveguide coupling for high-efficiency photon extraction

For the diamond nano-waveguides used in the Raman tuning and two-SiV entanglement experiments, we collect the Raman emission of SiV centers by adiabatically transferring the photons from the waveguide mode into a single-mode optical fiber (10). In this technique, a tapered optical fiber is brought into physical contact with a tapered section of a diamond waveguide. For an appropriate choice of the diamond and fiber geometries, the composite structure supports a single optical mode along its entire length, allowing a photon emitted by a SiV center inside the diamond waveguide to be transferred to the optical fiber. This technique can achieve high absolute coupling efficiencies and requires no realignment over the course of several days.

To achieve this goal, we use a wet-etching procedure to create conical tapers on conventional single-mode optical fibers (Thorlabs SM600) with a taper angle of approximately  $1.5^\circ$  (per side;  $3^\circ$  full angle). The triangular diamond waveguide is designed with a similar taper angle of  $2^\circ$ . Fiber coupling is achieved by positioning a tapered optical fiber in physical contact with the tapered section of the diamond waveguide using piezoelectric nanopositioners (Attocube ANPx101/ANPz101). The coupling efficiency from single-mode fiber to the diamond waveguide is calculated by sending light into a 90:10 fiber beamsplitter (Thorlabs TW670R5A2), with 90% of the input light sent to a reference photodiode (Thorlabs PDA100A), and the remaining 10% to the coupled fiber-waveguide structure. We use a Bragg mirror section of holes (similar to the mirror used to create the photonic crystal cavities above) in the waveguide to reflect the incoming light, 90% of which is sent to a calibrated measurement photodiode via the final beamsplitter port. By comparing the reflected power with the incoming power, we infer a lower bound on the fiber-diamond coupling efficiency of 70%.

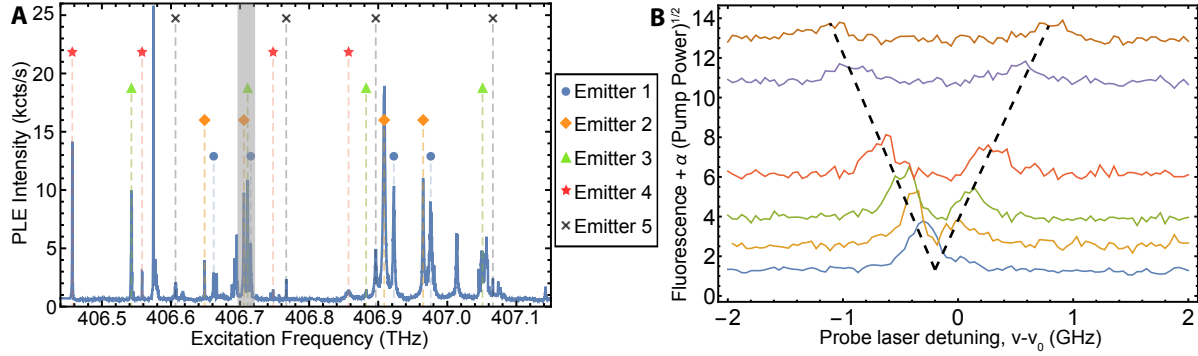

Figure S5: **(A)** Fluorescence counts from the center of the cavity as a function of excitation frequency. Colored symbols correspond to emitter frequencies determined by the algorithm described in the text. Emitters 1 and 2 are at low strain, and emitters 3–5 are at higher strain. The shaded region indicates a typical inhomogeneous distribution range of transition C ( $|c\rangle \leftrightarrow |e\rangle$ ) frequencies. The cavity QED experiments in the main text were carried out using Emitter 2. **(B)** The identification procedure was verified by measuring Autler-Townes splitting for the  $\Lambda$ -type system. A pump laser of varying intensity was fixed on transition D ( $|u\rangle \leftrightarrow |e\rangle$ ) at 406.649 THz, and a weak probe was scanned across transition C at 406.705 THz. The line splitting on transition C scales with the square root of the applied power on transition D (illustrated with dashed black line), confirming that the two transitions form an optical lambda system.

### 3 Identifying single SiV centers inside nanocavities

The electronic structure of the SiV center consists of spin-orbit doublets in the ground and excited states. Optical dipole transitions between the doublets result in four transition frequencies which are labeled A–D in order of decreasing frequency (11). The presence of strain in the crystal changes the energy splittings, resulting in inhomogeneous broadening (12). However, the difference in the transition frequencies always obeys the energy conservation constraints:  $\Delta_{A-B}^i = \Delta_{C-D}^i = \Delta_{gs}^i$  and  $\Delta_{A-C}^i = \Delta_{B-D}^i = \Delta_{es}^i$ , where  $\Delta_{es}^i$  and  $\Delta_{gs}^i$  are the excited and ground state splittings, corresponding to an individual emitter labeled  $i$ .

To determine the set of four transitions corresponding to a single emitter at the center of our cavity, we scanned the Ti:Sapphire laser over a 700 GHz range centered around 406.8 THz at  $\sim 100$  MHz resolution. We recorded the fluorescence counts in the PSB as a function of excitation frequency to obtain a list of all emitter resonances in this cavity. The resulting spectrum (Fig. S5A) indicates that there are several near-resonant SiV centers at the center of the cavity where each SiV results in four lines A–D<sup>*i*</sup>. We fit the frequency of each line in the Fig. S5A and calculate the energy differences  $\Delta$  between all pairs of lines. From this list, we find sets of four

frequencies  $A^i$ - $D^i$  that consist of pairs of transitions with matching  $\Delta$ , i.e.  $|\Delta_{A-B}^i - \Delta_{C-D}^i| < \epsilon$  where  $\epsilon \sim 300$  MHz is limited by experimental error in frequency estimation.

The results of this approach are indicated in Fig. S5A where we have drawn colored symbols over the sets of lines presumably corresponding to the same SiV. (Only five emitters are labeled.) To verify that these lines correspond to the same SiV, we apply a strong driving field on transition  $D^i$  ( $B^i$ ) and probe the response on transition  $C^i$  ( $A^i$ ). We observe that the probed transition undergoes a splitting proportional to the square root of the power of the driving field (Fig. S5B). This signature of the Autler-Townes effect confirms that the two transitions share an excited state as expected. When the two lines do not correspond to the same SiV, there is no observable splitting. For the optical switch experiment shown in Fig. 2 of the main manuscript, transitions C ( $|c\rangle \leftrightarrow |e\rangle$ ) and D ( $|u\rangle \leftrightarrow |e\rangle$ ) were used to realize an optical lambda system.

## 4 SiV charge state control: high fidelity initialization and single-shot readout

The SiV can be occasionally ionized from the  $\text{SiV}^-$  charge state to other charge states ( $\text{SiV}^0$  or  $\text{SiV}^{2-}$ ) which are dark in our measurement scheme. It is highly desirable to know when the SiV is in the correct charge state and to actively control the charge state. To accomplish these tasks, we performed the cavity transmission experiment in Fig. 1D with both the cavity and emitter on resonance with the probe laser. At first, only the weak, resonant probe laser was used for driving the system.

We recorded both the transmission photons collected through the cavity and the fluorescence photons collected in the phonon-sideband (PSB), and binned them in 15 ms intervals as shown in the blue curves in Fig. S6A. The SiV jumps between a bright state ( $\text{SiV}^-$ ) where the transmission intensity (thick blue trace) is low and the PSB fluorescence intensity (thin blue trace) is high and a dark state (not coupled to the probe field) with high transmission and no fluorescence. These jumps are clearly resolved on the timescale of seconds, allowing single-shot readout of the charge state of the SiV.

To rule out the possibility of faster ionization dynamics that we could not resolve with this slow technique, we performed a similar experiment but recorded the time-tagged photon arrival times with the fast acquisition electronics described above. We observed no features slower than tens of nanoseconds, indicating that the complete electronic dynamics are limited to those of the three-level optical system plus a slow charge switching process at the timescale of seconds

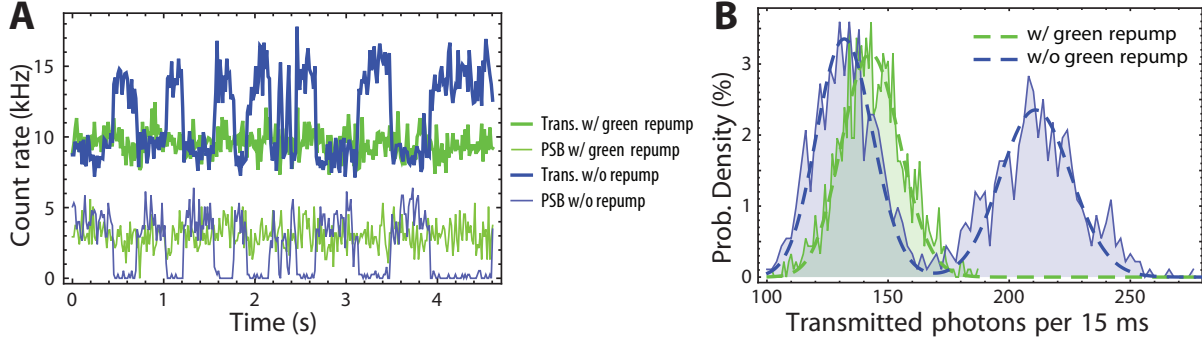

Figure S6: Charge state initialization with and without a green repump pulse. **(A)** Timetraces of transmission (upper thick curves) and phonon sideband (PSB, lower thin curves) photon detection events as a function of time. The data are taken both with (green) and without (blue) the presence of a 520 nm repump laser at approximately 10% duty cycle. Clear jumps are present in the case of no green repump, indicating single-shot readout of charge-state fluctuations. **(B)** Histograms of timetraces in A with Poissonian fits. The ratio of the two blue peak positions gives a direct measurement of the transmission dip of 37%. The mean number of transmitted photons in the case with green repump can be decomposed into 85% of the low-transmission peak and 15% of the high transmission peak in the case of no green repump. This implies an 85% charge state initialization fidelity.

for the laser intensities used in the experiment.

We then repeat the first experiment, with the addition of a  $10\ \mu\text{s}$  pulse of around 0.4 mW green light (520 nm) every  $100\ \mu\text{s}$ . The detectors are gated off during the green pulse. The time-traces recorded with this scheme (and with the same duty cycle and data processing as above) are shown in the green timetraces (thick: transmission, thin: PSB fluorescence) in Fig. S6A. These traces are flat and close to the values when the SiV is in the correct charge state, illustrating that there are no dynamics on the millisecond timescale and that the green pulse effectively repumps the SiV into the desired charge state.

To quantify this effect, we make histograms of photons detected per 15 ms bin for the transmission counts both with and without green repump (Fig. S6B). We fit a Poisson distribution to the histogram of counts taken with green repump and two Poisson distributions to the histogram of counts taken with no repump. Based on the relative amplitude of the two peaks without green repump, we estimate that the SiV is in the correct charge state 53% of the time. The average counts for the data taken with the green repump pulse can be decomposed into 85% of the low-transmission (SiV on) case and 15% of the high-transmission (SiV off) case, implying a charge-state initialization fidelity of 85%. A similar analysis using the PSB fluorescence has

more noise but is consistent with the above estimate. The close fit of these Poisson distributions to our data also indicates that there is no significant noise above shot noise on this timescale.

Finally, by measuring the contrast between the transmission counts in the bright and dark cases (i.e. the mean values of the peaks in Fig. S6B) we also have a simple and direct measurement of the transmission extinction from a single SiV. The value of the transmission dip extracted from this measurement is 37%, consistent with the measurement in Fig. 1F of the main manuscript. While the single-shot readout of the charge state shown in Fig. S6 can be used to initialize the system with near-perfect fidelity, further research is necessary to understand the microscopic mechanism for charge dynamics and develop higher fidelity control techniques.

## 5 Model description for a SiV center inside an optical cavity

In this section, we describe the theoretical model used to describe the dynamics of the SiV-cavity system measured in Figs. 1–3 of the main text. We show how to calculate the saturation response of the transmission and fluorescence of the system (Fig. 3A) and the different intensity correlation functions between detection events (Figs. 3B–D).

### 5.1 Three level dynamics with dissipation

The system is modeled by a three level atom inside a driven cavity as depicted in Fig. S7. In a

Figure S7: Setup for the coupled SiV-cavity system with dissipation.  $\xi/\sqrt{\kappa/2}$  is the flux amplitude of the weak coherent probe field, and  $\kappa$  is the total decay rate of the symmetric cavity. Dissipation channels are characterized by decay rates  $\gamma$ . The cavity drives the  $|c\rangle \leftrightarrow |e\rangle$  transition with a single-photon Rabi frequency  $g$  and a detuning  $\Delta_e$ .

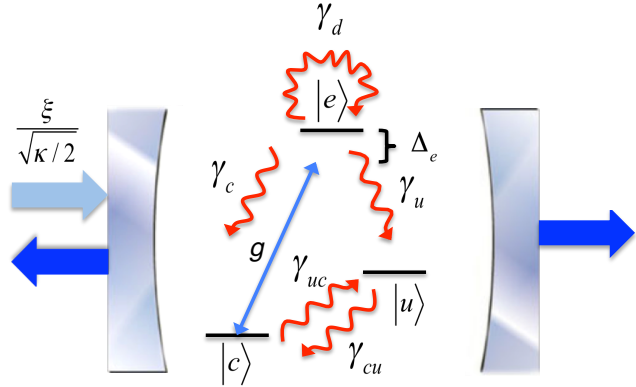

frame rotating with the probe frequency, the Hamiltonian is

$$\hat{H} = \Delta_e |e\rangle\langle e| + \Delta_c \hat{a}^\dagger \hat{a} + i\xi (\hat{a}^\dagger - \hat{a}) + ig (\hat{a}|e\rangle\langle c| - \hat{a}^\dagger |c\rangle\langle e|) \quad (1)$$

where  $\Delta_e = \omega_{ec} - \omega_p$ ,  $\Delta_c = \omega_c - \omega_p$ ,  $\omega_{ec}$  is the transition frequency between level  $|e\rangle$  and  $|c\rangle$ , and  $\omega_c$  is the resonance frequency of the cavity. The coupling between the cavity field and the SiV is given by the single-photon Rabi frequency  $g$ . The driving probe field is in a weak coherent state with a flux amplitude  $\xi/\sqrt{\kappa/2}$  and frequency  $\omega_p$ . The bosonic annihilation operator  $\hat{a}$  describes the cavity field. The dissipation in the system is described by the Lindblad operators

$$\begin{aligned}\hat{L}_1 &= \sqrt{\gamma_c}|c\rangle\langle e|, & \hat{L}_4 &= \sqrt{\gamma_{uc}}|u\rangle\langle c|, \\ \hat{L}_2 &= \sqrt{\gamma_u}|u\rangle\langle e|, & \hat{L}_5 &= \sqrt{\gamma_d}|e\rangle\langle e|, \\ \hat{L}_3 &= \sqrt{\gamma_{cu}}|c\rangle\langle u|, & \hat{L}_6 &= \sqrt{\kappa}\hat{a}\end{aligned}\tag{2}$$

where  $\gamma_{uc}$  and  $\gamma_{cu}$  are the nonradiative decay rates between states  $|c\rangle$  and  $|u\rangle$ ,  $\gamma_c$  ( $\gamma_u$ ) is the decay rate from state  $|e\rangle$  to state  $|c\rangle$  ( $|u\rangle$ ),  $\gamma_d$  is the dephasing rate of state  $|e\rangle$  and  $\kappa$  is the total decay rate of the cavity field. The Markovian approximation for the nonradiative relaxation rates ( $\gamma_{uc}, \gamma_{cu}, \gamma_d$ ) is justified by recent measurements of dephasing ( $\gamma_d$ ) and depolarization ( $\gamma_{cu}$ ) induced by a thermal phonon bath (13). Experimentally, we find that the optical transitions can be well described by Lorentzian profiles (see Fig. 2B), and that the slow non-Markovian dephasing (spectral diffusion) has a small contribution to the total linewidth.

The master equation describing the atom-cavity system can be written formally as

$$\dot{\rho} = -i[\hat{H}, \rho] + \sum_{x=1}^6 \hat{L}_x \rho \hat{L}_x^\dagger - \frac{1}{2} \left( \hat{L}_x^\dagger \hat{L}_x \rho + \rho \hat{L}_x^\dagger \hat{L}_x \right)\tag{3}$$

We work in the weak driving regime ( $\xi \ll \kappa$ ) and can therefore truncate the Hilbert space. To lowest order, we assume that at most two excitations are present in the system such that we can describe the system in the basis

$$\{|0, c\rangle, |0, e\rangle, |0, u\rangle, |1, c\rangle, |1, e\rangle, |1, u\rangle, |2, c\rangle, |2, u\rangle\}.\tag{4}$$

We label these states  $\{|1\rangle \dots |8\rangle\}$ .

## 5.2 System saturation response

To model the saturation response of the transmission and fluorescence measured in Fig. 3A, we look at the steady state of the system. For this calculation, we assume that the cavity is driven resonantly ( $\Delta_c = 0$ ) and we are in the regime where  $\kappa \gg g, \Delta_e, \xi, \gamma$  and  $g \gg \gamma$ . This makes it

possible to approximately solve the master equation for the steady state density matrix elements  $\rho_{i,j}^{(s)} = \langle i | \rho^{(s)} | j \rangle$  analytically. The expressions for  $\rho_{i,j}^{(s)}$  can be found in Sec. 9.1.

The transmission is then given by

$$\mathcal{T} = \frac{\kappa_b \langle \hat{a}^\dagger \hat{a} \rangle_s}{\langle \hat{a}_{\text{in}}^\dagger \hat{a}_{\text{in}} \rangle} \approx \frac{\kappa_a \kappa_b \left( \rho_{4,4}^{(s)} + \rho_{6,6}^{(s)} \right)}{\xi^2}, \quad (5)$$

where  $\kappa_a$  ( $\kappa_b$ ) describes the cavity decay rate to the input (output) waveguide mode. The total cavity decay rate is  $\kappa = \kappa_a + \kappa_b + \kappa'$ , where  $\kappa'$  is the loss rate out of the cavity not collected by the input and output waveguide modes. In our experiment, we use a waveguide damped symmetric cavity with  $\kappa_a \approx \kappa_b \approx \kappa/2$ .  $\langle \hat{a}_{\text{in}}^\dagger \hat{a}_{\text{in}} \rangle = 2\xi^2/\kappa$  is the photon flux of the input coherent state. The fluorescence scattering is given by

$$\mathcal{F} = \frac{\langle \sigma_{e,e} \rangle_s}{\langle \hat{a}_{\text{in}}^\dagger \hat{a}_{\text{in}} \rangle} \approx \frac{(\gamma_c + \gamma_u)\kappa}{2\xi^2} \left( \rho_{2,2}^{(s)} + \rho_{5,5}^{(s)} \right) \quad (6)$$

where  $\hat{\sigma}_{e,e} = |e\rangle\langle e|$ . We note that the observed saturation response differs from the two-level system response due to the presence of a second metastable level  $|u\rangle$ .

These expressions for  $\mathcal{T}$  and  $\mathcal{F}$  successfully capture the experimentally measured saturation response in fluorescence and transmission (see Fig. 3A) using the system parameters given in Section 5.4. In Fig. 3A, we express the photon flux,  $2\xi^2/\kappa$ , in terms of number of photons per Purcell-reduced excited-state lifetime  $\tau_e$ . The experimental data (dots) were fit to the theoretical curves (solid curves) using a single fit parameter for the scaling between the photon flux at the cavity (horizontal scale in the figure) and the photon detection rate. We find that a photon detection rate of approximately 110 kHz corresponds to a photon flux of 1 photon per lifetime. This scaling parameter accounts for the detection efficiency in the experiment, and the fit result is in agreement with our independent estimates of the detection efficiency ( $\sim 10^{-4}$ ).

### 5.3 Calculation of intensity correlation functions

In order to calculate the intensity correlation functions measured in Fig. 3, we need to evaluate the response of the system following the detection of either a cavity photon or a scattered photon. Since we work below saturation, the evolution of the metastable states ( $|0, c\rangle$ ,  $|0, u\rangle$ ) are approximately determined solely by the dissipative coupling between these two states such that

$$\dot{\rho}_{1,1} \approx \gamma_{cu}\rho_{3,3} - \gamma_{uc}\rho_{1,1} \quad (7)$$

$$\dot{\rho}_{3,3} \approx \gamma_{uc}\rho_{1,1} - \gamma_{cu}\rho_{3,3}. \quad (8)$$

This can be solved to yield  $\rho_{1,1}(t) = \alpha + \beta e^{-\tilde{\gamma}t}$ ,  $\rho_{3,3}(t) = \alpha_2 - \beta e^{-\tilde{\gamma}t}$ , where  $\alpha = \frac{\gamma_{cu}(\rho_{1,1}(0) + \rho_{3,3}(0))}{\tilde{\gamma}}$ ,  $\beta = \frac{\gamma_{uc}\rho_{1,1}(0) - \gamma_{cu}\rho_{3,3}(0)}{\tilde{\gamma}}$ ,  $\alpha_2 = \frac{\gamma_{uc}(\rho_{1,1}(0) + \rho_{3,3}(0))}{\tilde{\gamma}}$  and  $\tilde{\gamma} = \gamma_{cu} + \gamma_{uc}$ . In steady state, the populations are given by  $\rho_{1,1}^{(s)} \approx \gamma_{cu}/(\gamma_{cu} + \gamma_{uc})$  and  $\rho_{3,3}^{(s)} \approx \gamma_{uc}/(\gamma_{cu} + \gamma_{uc})$ . The ratio of  $\gamma_{uc}/\gamma_{cu}$  is determined by the thermal distribution (13). Using data from the optical pumping experiment shown in Fig. 2, we infer  $\rho_{1,1} \sim 64\%$  and  $\rho_{3,3} \sim 36\%$  in steady state. These values are in good agreement with a thermal distribution of population at 4K for the two metastable states that are split by 64 GHz.

Using these expressions for the metastable state populations, we can analytically solve the equations of motion for the populations in the other levels to the leading order in the probe field amplitude. We use the assumption of weak resonant driving ( $\Delta_c = 0$ ) and that we are in the bad cavity regime ( $\kappa \gg g \gg \gamma \gg \xi$ ), to identify the dominant terms and adiabatically eliminate all states containing cavity photons. As a result, we are left with only three coupled differential equations that we need to solve between  $\dot{\rho}_{2,2}$  and  $\dot{\rho}_{1,2}, \dot{\rho}_{2,1}$ . Solving the equations, we end up with the following expressions:

$$\rho_{1,2}(t) \approx \mathcal{A}_1 + \mathcal{A}_2 e^{-\tilde{\gamma}t} + \mathcal{A}_3 e^{a_1 t}, \quad \rho_{6,6}(t) \approx \frac{4\xi^2}{\kappa^2} \rho_{3,3}(t), \quad (9)$$

$$\rho_{2,2}(t) \approx \mathcal{B}_1 + \mathcal{B}_2 e^{-\tilde{\gamma}t} + \mathcal{B}_3 e^{a_1 t} + \mathcal{B}_4 e^{b_1 t}, \quad \rho_{7,7}(t) \approx \frac{4(\xi^2 \rho_{4,4}(t) + g^2 \rho_{5,5}(t))}{3\kappa^2} \quad (10)$$

$$\rho_{4,4}(t) \approx \mathcal{C}_1 + \mathcal{C}_2 e^{-\tilde{\gamma}t} + \mathcal{C}_3 e^{a_1 t} + \mathcal{C}_4 e^{b_1 t}, \quad \rho_{8,8}(t) \approx \frac{6\xi^2}{3\kappa^2} \rho_{6,6}(t), \quad (11)$$

$$\rho_{5,5}(t) \approx \frac{4\xi^2}{\kappa^2} \rho_{2,2}(t). \quad (12)$$

The coefficients  $a_i$ ,  $b_i$ ,  $\mathcal{A}_i$ ,  $\mathcal{B}_i$  and  $\mathcal{C}_i$  are defined in Sec. 9.2.

From Eqs. (9)–(12), it is straightforward to get the steady state population of the different levels by taking the limit  $t \rightarrow \infty$ . From the steady state populations we can calculate  $\langle \hat{a}^\dagger \hat{a} \rangle \approx \rho_{4,4}^{(s)} + \rho_{6,6}^{(s)}$  and  $\langle \hat{\sigma}_{e,e} \rangle \approx \rho_{2,2}^{(s)}$ . The normalized transmission–transmission intensity correlation function (Fig. 3C) is given by

$$g_{TT}^{(2)}(\tau) = \frac{\langle \hat{a}^\dagger(0) \hat{a}^\dagger(\tau) \hat{a}(\tau) \hat{a}(0) \rangle}{\langle \hat{a}^\dagger \hat{a} \rangle^2}, \quad (13)$$

where  $\langle \hat{a}^\dagger(0) \hat{a}^\dagger(\tau) \hat{a}(\tau) \hat{a}(0) \rangle \approx \rho_{4,4}(\tau) + \rho_{6,6}(\tau)$  can be calculated from Eqs. (9) and (11) with initial conditions given by the detection of a cavity photon at time  $t = 0$ , i.e.  $\rho(0) = \hat{a} \rho^{(s)} \hat{a}^\dagger$ . Consequently,  $\rho_{1,1}(0) = \rho_{4,4}^{(s)}$ ,  $\rho_{3,3}(0) = \rho_{6,6}^{(s)}$ ,  $\rho_{2,2}(0) = \rho_{5,5}^{(s)}$  and  $\rho_{1,2}(0) = (4\xi^2 \rho_{1,2}^{(s)} + 2\xi g \rho_{4,4}^{(s)} - 4\xi g \rho_{2,2}^{(s)})/\kappa^2$ . The normalized intensity autocorrelation function for the scattered (fluorescence)

field (see Fig. 3B)

$$g_{SS}^{(2)}(\tau) = \frac{\gamma_u^{(rad)}}{\gamma_c^{(rad)} + \gamma_u^{(rad)}} \frac{\langle \hat{\sigma}_{e,u}(0) \hat{\sigma}_{e,e}(\tau) \hat{\sigma}_{u,e}(0) \rangle}{\langle \hat{\sigma}_{e,e} \rangle^2} + \frac{\gamma_c^{(rad)}}{\gamma_c^{(rad)} + \gamma_u^{(rad)}} \frac{\langle \hat{\sigma}_{e,c}(0) \hat{\sigma}_{e,e}(\tau) \hat{\sigma}_{c,e}(0) \rangle}{\langle \hat{\sigma}_{e,e} \rangle^2}, \quad (14)$$

and the normalized intensity correlation function between the scattered and transmitted fields (see Fig. 3D)

$$g_{ST}^{(2)}(\tau = \tau_F - \tau_T > 0) = \frac{\langle \hat{a}^\dagger(0) \hat{\sigma}_{e,e}(\tau) \hat{a}(0) \rangle}{\langle \hat{a}^\dagger \hat{a} \rangle \langle \hat{\sigma}_{e,e} \rangle} \quad (15)$$

$$g_{ST}^{(2)}(\tau < 0) = \frac{\gamma_u^{(rad)}}{\gamma_c^{(rad)} + \gamma_u^{(rad)}} \frac{\langle \hat{\sigma}_{e,u}(0) \hat{a}^\dagger(-\tau) \hat{a}(-\tau) \hat{\sigma}_{u,e}(0) \rangle}{\langle \hat{a}^\dagger \hat{a} \rangle \langle \hat{\sigma}_{e,e} \rangle} + \frac{\gamma_c^{(rad)}}{\gamma_c^{(rad)} + \gamma_u^{(rad)}} \frac{\langle \hat{\sigma}_{e,c}(0) \hat{a}^\dagger(-\tau) \hat{a}(-\tau) \hat{\sigma}_{c,e}(0) \rangle}{\langle \hat{a}^\dagger \hat{a} \rangle \langle \hat{\sigma}_{e,e} \rangle}, \quad (16)$$

can be calculated in a similar way where  $\hat{\sigma}_{u,e} = |u\rangle\langle e|$  and  $\hat{\sigma}_{c,e} = |c\rangle\langle e|$ . Equations (15) and (16) correspond to cases where a transmitted or a scattered photon was detected first, respectively. Note that for correlations involving the fluorescence field, detection of photons emitted in  $|e\rangle \rightarrow |u\rangle$  (detection probability  $\sim \gamma_u^{(rad)}$ ) or  $|e\rangle \rightarrow |c\rangle$  (detection probability  $\sim \gamma_c^{(rad)}$ ) can result in different dynamics and two separate terms. While these photons (or two paths) are in principle distinguishable by frequency, in our experiment both paths were detected without frequency filtering. For this reason, a photon detection in fluorescence leaves the SiV in some classical mixture of states  $|c\rangle$  (with probability  $\gamma_c^{(rad)} / (\gamma_c^{(rad)} + \gamma_u^{(rad)})$ ) and  $|u\rangle$  (with probability  $\gamma_u^{(rad)} / (\gamma_c^{(rad)} + \gamma_u^{(rad)})$ ). On the other hand, the detection of a cavity photon preferentially leaves the SiV in state  $|u\rangle$ . This results in the asymmetry in the fluorescence–transmission intensity cross-correlation function measured in Fig. 3D.

## 5.4 Extraction of system parameters

The data shown in Figs. 1–3 of the main manuscript can be modeled using a single set of intrinsic system parameters. The cavity decay rate  $\kappa$  is measured from the envelope of the cavity transmission curve in Fig. 1E (blue curve). The dephasing rate  $\gamma_d$  of the SiV optical transition ( $|c\rangle \rightarrow |u\rangle$ ) is measured from the SiV linewidth in Fig. 1F when the cavity is off resonance with the SiV (orange curve), while the single-photon Rabi frequency  $g$  is determined

by the Purcell-broadened linewidth when the cavity is on resonance with the SiV (red curve). These values are consistent with the independent time-domain lifetime measurement described in the main text. These values (which suffice to determine the cooperativity) are then taken as fixed; the remaining parameters are extracted from the photon correlation measurements in Figs. 3C and 3D. (The data in Fig. 3B were taken above saturation with large cavity detuning ( $\Delta_e = 0, \Delta_c \gg \kappa$ ) and were modeled separately as a three-level atom in a classical field.) The optical switching experiment (Fig. 2) provides an independent measurement of the ground-state relaxation rates  $\gamma_{uc}$  and  $\gamma_{cu}$  and is consistent with the values extracted from the photon correlation measurements.

The following parameters (defined in Fig. S7) accurately describe the system dynamics:  $\{\kappa = 1150 \gamma_0, \gamma_d = 4 \gamma_0, \gamma_u = \gamma_0, \gamma_c = \gamma_0, \gamma_{uc} = 0.10 \gamma_0, \gamma_{cu} = 0.15 \gamma_0, g = \gamma_0 (1.5\kappa/\gamma_0)^{1/2}, \gamma_c^{(rad)}/\gamma_u^{(rad)} = 2\}$  where we defined  $\gamma_0 = 2\pi \times 50$  MHz. Of these parameters,  $\{\kappa, \gamma_d, \gamma_{uc}, \gamma_{cu}, g\}$  are consistent with independently measured values in Figs. 1–3. The detected ratio of  $\gamma_c^{(rad)}/\gamma_u^{(rad)}$  determines the asymmetry of  $g_{ST}^2(\tau)$  and was fit separately using the data in Fig. 3D. The theoretical expressions for photon correlations were convolved with the detector timing response (300 ps timing jitter per APD) to obtain the solid curves in Fig. 3. Intensity correlation measurements were normalized using intensity averages; we do not observe excess noise due to incoherent dynamics at slow timescales.

## 5.5 Measured vs. expected cooperativity

Our measured cooperativity of  $C \sim 1$  differs substantially from the cooperativity  $C = \frac{4g^2}{\kappa\gamma} = \frac{3}{4\pi^2} \frac{Q}{V} \left(\frac{\lambda}{n}\right)^3 \sim 275$  in the ideal case of a perfect emitter coupled optimally to our cavity with measured quality factor  $Q \sim 7200$  and dimensionless mode volume  $\frac{V}{(\lambda/n)^3} \sim 3$ . In this section, we discuss the discrepancies leading to this disagreement.

First, the emitter is not optimally aligned with the cavity mode. Based on the crystallographic orientation of our sample and the electric field mode profile inside the cavity, the maximal overlap between the atomic transition dipole and the cavity mode is roughly 2/3. The positioning of the SiV center can be a separate source of error. The accuracy of FIB-based implantation (Section 2.5) is around 40 nm, including straggle. This is a significant fraction of the spatial extent of the local cavity field antinode that extends in about 100 nm in all three dimensions. This positioning error can reduce the atom–photon coupling and hence the cooperativity by roughly 20–40%.

In addition to reductions in the cooperativity due to emitter positioning errors, the SiV is

$$\begin{array}{c}
\begin{array}{ccc}
\text{cavity properties} & \text{atomic properties} & \text{atomic position and orientation} \\
\hline
C = \frac{3}{4\pi^2} \left( \frac{\lambda_0}{n} \right)^3 \frac{Q}{V} & \frac{\gamma_{ZPL}^{(rad)}}{\gamma^{(rad)}} \frac{\gamma_0}{\gamma_{exp}} \text{QE} & \left( \begin{array}{c} \text{dipole} \\ \text{orient.} \end{array} \right) \left( \begin{array}{c} \text{SiV} \\ \text{position} \end{array} \right) \\
C \approx \frac{1}{13} \frac{7200}{3} & 0.7 \quad 0.3 \text{ QE} & 0.4\text{--}0.8 \quad 0.4\text{--}1 \quad \sim 10 \times \text{QE}
\end{array}
\end{array}$$

Table 1: Cooperativity estimate based on SiV and experimental parameters described in the text

not a perfect optical emitter. The atomic decay rate  $\gamma$  in the cooperativity includes all photon emission and decoherence rates, whereas the single-photon Rabi frequency  $g$  includes only the contribution from the dipole transition ( $|c\rangle \leftrightarrow |e\rangle$ ) that couples to the cavity mode. The cooperativity is therefore reduced by imperfections in the optical transitions of the SiV center. First, the Debye-Waller factor ( $\gamma_{ZPL}^{(rad)}/\gamma^{(rad)}$ ) for the SiV ZPL is around 70%. Next, our linewidth is broadened by phonon processes and spectral diffusion to approximately three times the lifetime-limited linewidth ( $\gamma_0/\gamma_{exp} \approx 0.3$ ). For the lambda system used in the experiment, the branching ratio of the  $|e\rangle \rightarrow |c\rangle$  and  $|e\rangle \rightarrow |u\rangle$  ZPL transitions are about 80% and 20% respectively (14). Finally, if there is a significant nonradiative decay rate limiting the quantum efficiency (QE) of the SiV, our observed cooperativity could be substantially reduced.

Taking conservative estimates for the parameters other than an unknown quantum efficiency, our estimated cooperativity is around  $C \sim 10 \times \text{QE}$  (Table 1). A quantum efficiency of around 10% is therefore consistent with the discrepancy between our expected and observed cooperativity.

## 6 Subnatural-linewidth Raman single photons

The Raman tuning demonstrated in Fig. 4 uses off-resonant laser excitation to generate spectrally-tunable subnatural linewidth single photons. In this section, we discuss technical considerations that enable us to isolate single photons under off-resonant excitation and present data that support our claims about subnatural linewidths for Raman photons. The SiV centers used for the Raman tuning and entanglement experiments have a ground state frequency splitting of  $\approx 50$  GHz. When we excite the  $|u\rangle \rightarrow |c\rangle$  transition with a laser at frequency  $\nu$ , the Raman photons are at a frequency  $\approx \nu + 50$  GHz. We use separate spatial modes for laser excitation (free-space, see Fig. 4) and Raman photon detection (waveguide mode collected via fiber). This allows us to significantly suppress leakage from the excitation laser into our collection mode.

Despite this suppression, the scattering at the diamond-vacuum interface results in laser leakage into the collection mode. When we excite the  $|u\rangle \rightarrow |c\rangle$  transition on resonance, we find that the typical signal to noise ratio between the Raman single-photons and laser background is about  $\sim 1$ .

To obtain Raman single-photons with high purity, we use a home-built scanning Fabry-Perot (FP) filter cavity designed to have high transmission for Raman photons at frequency  $\approx \nu + 50$  GHz while suppressing laser photons at frequency  $\nu$ . To achieve this, we built a cavity with a free spectral range (FSR) of 37 GHz which maximally suppresses the laser field (by putting the laser line in the middle of the FSR, exactly between two cavity resonances) while maintaining a high cavity bandwidth of 150 MHz (FWHM, ringdown time 1.05 ns). We note that the high bandwidth is necessary to be able to measure the dynamics observed at the  $\approx 2.5$  ns timescale in Fig. 5D. The fit functions used for the data in Fig. 5D are convolved with the combined timing response of the cavity and the detectors.

The use of the FP cavity allows us to obtain a signal to noise ratio of  $\sim 1000$  under resonant excitation. At increased detunings  $\Delta$ , the scattering cross section of the SiV reduces according to  $\sim \frac{1}{(\Gamma/2)^2 + \Delta^2}$ , where  $\Gamma$  is the  $|u\rangle \leftrightarrow |e\rangle$  transition linewidth. This scaling is confirmed with the measurements shown Fig. S8A where we measure the Raman emission intensity at different detunings for a fixed laser power. The reduced scattering cross section at large detunings necessitates an increased laser power to maintain a fixed photon scattering and detection rate. The extinction ratio of the FP cavity ( $\sim 10^4$  for current device) is therefore a crucial parameter that sets the practical limit on the extent of Raman tuning. With the cavity used in the experiments, we are able to tune the Raman photons by 10 GHz in each direction while maintaining a signal to noise ratio above 1 (see extended data in Fig. S8C). The tuning range could be further extended by using a higher finesse cavity (or a second filter cavity) or cavity-enhanced Raman scattering.

Under off-resonant excitation with  $\Omega, \Gamma \ll \Delta$ , the linewidth of the Raman photons is determined by the coherence between the metastable states  $|u\rangle$  and  $|c\rangle$ . In this limit, it is therefore possible to achieve subnatural linewidth photons, that is, photons that are narrower than the natural spontaneous emission linewidth of 90 MHz (corresponding lifetime  $\tau_e \approx 1.8$  ns). When we measure the linewidth of the Raman photons in Fig. S8B, we find that the linewidth is limited by the resolution of the FP cavity 180 MHz. When we use a different FP cavity with a resolution of 30 MHz, we find that the Raman linewidth is less than 30 MHz (inset of Fig. S8B), demonstrating subnatural-linewidth Raman photon emission.

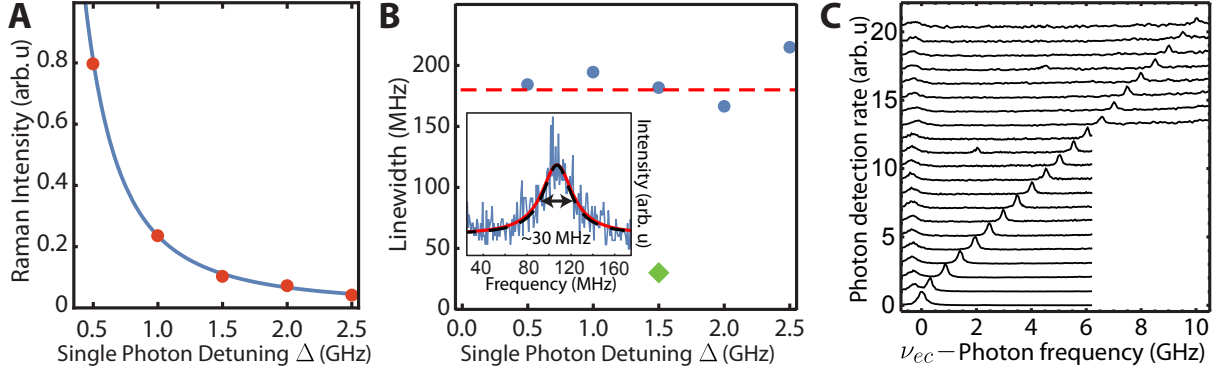

Figure S8: **(A)** Raman fluorescence intensity for a fixed laser power measured at different single photon detunings  $\Delta$ . The solid line is a fit with the form  $\frac{A}{(\Gamma/4\pi)^2 + (\Delta)^2}$  with  $\Gamma/2\pi = 440$  MHz. **(B)** Raman emission linewidth as a function of detuning. At all detunings, the Raman emission linewidth (blue circles) is limited by the cavity linewidth (dashed red line). When a narrow-linewidth cavity with FWHM  $\sim 30$  MHz is used to measure the Raman linewidth, the linewidth is significantly narrower (green diamond). Inset: Raman fluorescence intensity as a function of narrow-linewidth cavity frequency. The fitted Lorentzian response (solid red curve) is almost identical to the measured cavity transfer function (dashed black curve) indicating that the Raman linewidth is less than the 30 MHz cavity bandwidth. **(C)** Extended data for Fig. 4C, showing Raman tuning over 10 GHz on the red sideband.

## 7 Experimental procedure for entanglement generation

To generate entanglement between two SiV centers, we perform the same Raman tuning technique simultaneously on two spatially-separated SiV centers in a single diamond waveguide. The waveguide is again adiabatically coupled to a single-mode optical fiber as described in Sec. 2.6. The collected photons are frequency filtered (see below) and then sent to a Hanbury Brown-Twiss setup to measure the photon autocorrelation function using the detectors and electronics described in Sec. 1. The theoretical analysis of the system will be presented in Sec. 8.

For the photon autocorrelation measurements performed when the two SiV centers are Raman-tuned onto resonance (Fig. 5B, red curve in Fig. 5D), the Raman fluorescence from both SiV centers passes through the FP cavity (FWHM: 150 MHz, FSR: 37 GHz, Transmission: 80%), ensuring frequency indistinguishability. For the two SiVs used in the entanglement experiment, the transition frequencies  $\nu_{ec}$  were detuned by about 1 GHz. The emitters were excited below saturation using two frequency stabilized lasers at single photon detunings  $\Delta_1 = 1.3$  GHz for SiV1 and  $\Delta_2 = 2.3$  GHz for SiV2, and the Raman emission frequencies and intensities were matched. During the course of the measurement, the Raman emission fre-

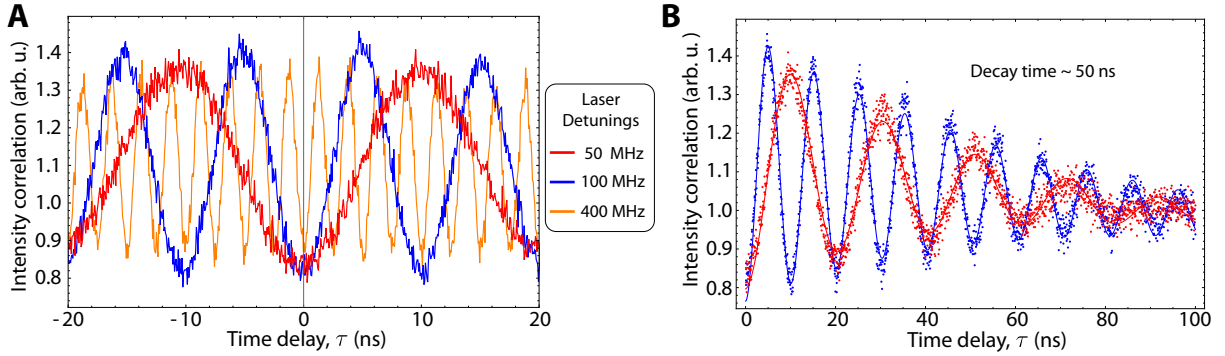

Figure S9: Phase stability of the two Raman excitation lasers. The two lasers are combined on a beamsplitter and the intensity correlations are measured at the two output ports. **(A)** When the two lasers are detuned, intensity beats are observed. For the timescales considered in the entanglement experiment ( $\tau < 10$  ns, see Fig. 5D), the laser beats do not decay and the relative phase of the two lasers is stable. **(B)** The laser beats decay at a longer timescale of  $\sim 50$  ns that is determined by the relative linewidths of the two lasers.

quency for the SiV centers underwent slow spectral drifts of order 100 MHz at the  $\sim 10$  minute timescale that were compensated by the frequency of the excitation lasers. In other words, effects of slow spectral diffusion were mitigated using the Raman tuning technique. The Raman emission rates into the waveguide mode from each SiV were independently monitored to assure balanced emission. For these measurements, it is also important that the relative phase of the two driving lasers does not drift over the  $\sim 10$  ns lifetime of the entangled state (see Sec. 8.1 for a theoretical discussion). This requirement is fulfilled by the frequency stabilization scheme described in Sec. 1. We experimentally verify the relative phase stability of the two driving fields by performing a time-domain interference measurement (Fig. S9).

For the autocorrelation measurements performed in the distinguishable case (Fig. 5C, blue curve in Fig. 5D), the frequencies of the Raman photons from the two SiV centers are not tuned on resonance and differ by about 1 GHz. In this measurement, we split the fluorescence from the two SiV centers using a 50/50 beamsplitter and send each path to a separate FP cavity: FP1 (FWHM: 150 MHz, FSR: 37 GHz, Transmission: 80%) is tuned to SiV1 Raman emission, FP2 (solid etalon with FWHM: 800 MHz, FSR: 20.3 GHz, Transmission: 80%) is tuned to SiV2 Raman emission. The two paths are then recombined on a second 50/50 beamplitter and sent to two detectors to measure photon correlations.

## 8 Model description for entanglement in a two-SiV system

In this Section, we analyze entanglement generation and verification for two SiV centers coupled to a waveguide. Specifically, we first use a simple model to describe the two-SiV entanglement generation process (Sec. 8.1). We next extend this model in Sec. 8.2 to include dissipation and show that it can be used to describe the observations reported in the main text. We next present the analyses showing that how the photon correlation measurements can be used to verify entanglement generation. Specifically, in Sec. 8.3.1, we derive an expression for the concurrence of the two-SiV system after detection of a single photon. We show that the concurrence is positive, demonstrating the presence of entanglement conditioned on detection of a single photon. In Sec. 8.3.2, we use a more specific model for our system to estimate the fidelity of the entangled state  $|B\rangle$  conditioned on detection of two photons within a short time delay. The resulting fidelity also demonstrates creation of an entangled state.

### 8.1 Simple model

The process of entanglement generation can be understood through a simple model of the system. The two SiVs in the waveguide can be modeled as two three-level systems in a lossy cavity as in Sec. 5. In a proper rotating frame, the Hamilton of the system is

$$\begin{aligned} \hat{H} = & \Delta_1|e\rangle_1\langle e| + \Delta_2|e\rangle_2\langle e| + (\Omega_1|e\rangle_1\langle u| + \Omega_2|e\rangle_2\langle u| + h.c.) \\ & + (g_1|e\rangle_1\langle c|\hat{a} + g_2|e\rangle_2\langle c|\hat{a} + h.c.), \end{aligned} \quad (17)$$

where we have assumed that both Raman transitions are on resonance and defined  $\Delta_i = \omega_{ei} - \omega_{Li}$  where  $\omega_{ei}$  is the frequency of level  $|e\rangle_i$  and  $\omega_{Li}$  is the frequency of the laser associated with the coupling  $\Omega_i$ , which we assume to be real. The photonic operator  $\hat{a}$  describes the single mode field that both emitters couple to. Since we are operating in the far detuned regime, we can adiabatically eliminate the excited states, which results in an effective Hamiltonian

$$\hat{H}_{\text{eff}} \approx -\tilde{g}_1\hat{\sigma}_{uc}^{(1)}\hat{a} - \tilde{g}_2\hat{\sigma}_{uc}^{(2)}\hat{a} + h.c. \quad (18)$$

where  $\tilde{g}_i \approx \frac{\Omega_i g_i}{\Delta_i}$  and we have defined  $\hat{\sigma}_{uc}^{(i)} = |u\rangle_i\langle c|$ . We have neglected any shifts of the ground states due to laser and cavity couplings since we are far detuned.

To understand entanglement generation, we consider the initial state of the SiVs  $|u\rangle_1|u\rangle_2$  since this is the only state that can emit two Raman photons. The evolution of this initial state

under the above Hamiltonian is

$$U(\epsilon)|u\rangle_1|u\rangle_2|0\rangle \approx |u\rangle_1|u\rangle_2|0\rangle + i\epsilon(\tilde{g}_1|c\rangle_1|u\rangle_2 + \tilde{g}_2|u\rangle_1|c\rangle_2)|1\rangle, \quad (19)$$

where  $U(t) = e^{-i\hat{H}t}$ ,  $|0\rangle$  ( $|1\rangle$ ) is the vacuum (single photon) state of the waveguide mode and we have expanded the time evolution assuming that we are looking at a time  $\epsilon \ll 1/\tilde{g}_{1,2}$ . In the experiment, the strength of the lasers is tuned such that  $|\tilde{g}_1| = |\tilde{g}_2| = \tilde{g}$  and we write  $g_2 = g_1 e^{i\phi}$  where  $\phi$  results from the propagation phase between the emitters in the waveguide and the relative phase of the two driving lasers. As described above, the two driving lasers are frequency stabilized such that the phase  $\phi$  is constant over timescales much longer than any other system dynamics. Under these conditions, we have

$$U(\epsilon)|u\rangle_1|u\rangle_2|0\rangle \approx |u\rangle_1|u\rangle_2|0\rangle + i\epsilon\tilde{g}(|c\rangle_1|u\rangle_2 + e^{i\phi}|u\rangle_1|c\rangle_2)|1\rangle. \quad (20)$$

The detection of the first photon thus prepares the SiVs in the entangled state

$$|B\rangle = (|c\rangle_1|u\rangle_2 + e^{i\phi}|u\rangle_1|c\rangle_2)/\sqrt{2}. \quad (21)$$

This state  $|B\rangle$  is a superradiant state, which emits photons at a rate which is twice that of a single emitter in state  $|u\rangle$ . This can be seen from the evolution of this state under the Hamiltonian in Eq. (18):

$$U(\epsilon)|B\rangle|0\rangle \approx |B\rangle|0\rangle - \sqrt{2}i\epsilon\tilde{g}e^{i\phi}|c\rangle_1|c\rangle_2|1\rangle. \quad (22)$$

The  $\sqrt{2}$  prefactor of  $|c\rangle_1|c\rangle_2|1\rangle$  corresponds to a factor of 2 enhancement of the emission rate compared to that of a single emitter in state  $|u\rangle$ . It is this enhanced emission rate that results in the measured peak in the normalized photon correlation function  $g^{(2)}$  at zero delay time in Fig. 5D.

## 8.2 Detailed model

We next present a more detailed model of the waveguide experiment including various dissipation channels in order to model the time-dependent  $g^{(2)}$ -correlation functions. We describe the unitary dynamics using Eq. (17) and the dissipation in the system using the Lindblad operators defined in Eq. (2) for each atom. The only exception is that we now define  $\hat{L}_{5,i} = \sqrt{\gamma_d}|u\rangle_i\langle u|$  because we scatter Raman photons at a large detuning ( $\Delta_i \gg \gamma_u$ ) where the contribution from excited state dephasing can be neglected and ground state dephasing dominates. Furthermore,

we assume that the two atoms have equal decay rates. Since  $\Delta_i \gg \Omega_i, g_i$ , we can again adiabatically eliminate the excited states, which results in the effective Hamiltonian in Eq. (18). The effective Lindblad operators are  $\hat{L}_{3,i}$  through  $\hat{L}_{6,i}$  and

$$\hat{L}_{1,i}^{\text{eff}} \approx \frac{\sqrt{\gamma_c}}{\Delta_i} (\Omega_i |c\rangle_i \langle u| + g_i |c\rangle_i \langle c|\hat{a}) \quad (23)$$

$$\hat{L}_{2,i}^{\text{eff}} \approx \frac{\sqrt{\gamma_u}}{\Delta_i} (\Omega_i |u\rangle_i \langle u| + g_i |u\rangle_i \langle c|\hat{a}). \quad (24)$$

Since we operate in the weak-driving regime, we can truncate the Hilbert space assuming that at most two photons are present in the system. In this case, the system can be described in a basis of the states

$$\left\{ |uu\rangle|0\rangle, |uc\rangle|0\rangle, |cu\rangle|0\rangle, |cc\rangle|0\rangle, |uu\rangle|1\rangle, |uc\rangle|1\rangle, |cu\rangle|1\rangle, |cc\rangle|1\rangle, |uu\rangle|2\rangle, |uc\rangle|2\rangle, |cu\rangle|2\rangle, |cc\rangle|2\rangle \right\}, \quad (25)$$

which we label  $\{|1\rangle, \dots, |12\rangle\}$ . The notation is such that  $|uc\rangle|1\rangle$  denotes atomic state  $|u\rangle_1|c\rangle_2$  and one photon in mode  $\hat{a}$ . In this basis, we can solve the master equation for the system by adiabatically eliminating all states containing cavity photons since the cavity mode is in this experiment a simple waveguide and therefore has extremely fast decay. We also assume that the dynamics of the ground states  $\{|1\rangle, \dots, |4\rangle\}$  are governed solely by the dissipative couplings between them (similar to the procedure in Sec. 5.3) since we are in the weak driving regime and that  $|g_i|^2/(\kappa\gamma_u) \ll 1$ .

Under these conditions, we find that the photon intensity correlation function can be expressed as

$$g^{(2)}(\tau) \approx \frac{(\alpha_1 + \alpha_2)\rho_{1,1}(\tau) + \alpha_1\rho_{2,2}(\tau) + \alpha_2\rho_{3,3}(\tau) + 2\alpha_3\rho_{2,3}(\tau)}{\left((\alpha_1 + \alpha_2)(\rho_{1,1}^{(s)} + \rho_{2,2}^{(s)})\right)^2}, \quad (26)$$

where  $\rho_{i,j} = \langle i|\rho|j\rangle$  and  $\rho^{(s)}$  denotes the steady state density matrix of the system and  $\rho = \hat{a}\rho^{(s)}\hat{a}^\dagger$ . The matrix elements and constants are defined in Sec. 9.3. The peak in the  $g^{(2)}$  function at zero time-delay originates from the coherence  $\alpha_3\rho_{2,3}(\tau)$  between the two ground states. This is consistent with the simple model description in Sec. 8.1: If the laser strengths are tuned such that  $\left|\frac{\Omega_1^*g_1}{\Delta_1}\right| = \left|\frac{\Omega_2^*g_2}{\Delta_2}\right|$  and  $g_2 = g_1e^{i\phi}$  then  $\rho_{1,1}(0) = 0$  and  $\alpha_1\rho_{2,2}(0) = \alpha_2\rho_{3,3}(0) = \alpha_3\rho_{2,3}(0)$ , which means that the peak is a result of the enhanced emission rate of the entangled state  $|B\rangle$ . The coherence  $\rho_{2,3}(\tau)$  decays with a rate  $\Gamma \approx \gamma_{cu} + \gamma_{uc} + \gamma_d$ , which determines the width of the peak.

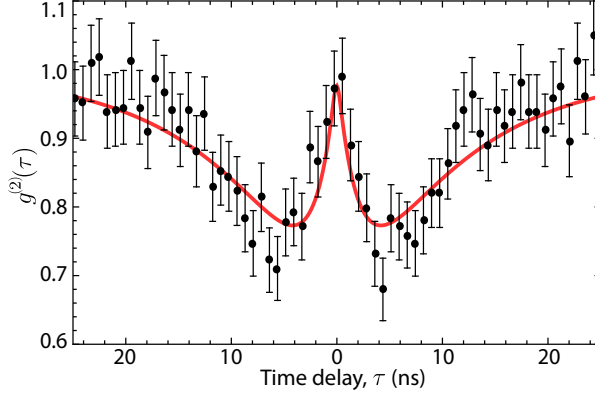

Figure S10: Comparison of model (solid red curve) to data (black points) using the following parameters (defined in Eq. (2)):  $\{\Delta_1, \Delta_2, \gamma_{cu}, \gamma_{uc}, \gamma_{uu}, \Omega_1, \Omega_2\} = \{22, 14, 0.10, 0.06, 0.66, 0.23, 0.15\} \times \gamma_0$  with  $\gamma_0 = 2\pi \times 94$  MHz. The model has been convolved with a Gaussian to account for the finite detector jitter present in the experiment. Of these parameters,  $\Delta_1$ ,  $\Delta_2$  and the odds of detecting a noise photon  $p_n = 0.09$  are fixed based on single-photon detunings and single SiV  $g^{(2)}$  measurements; the other parameters are estimated by fitting the data to the model under conservative physical constraints. The data correspond to the red curve in Fig. 5D in the main text.

Eq. (26) corresponds to the ideal limit where no noise photons, e.g. originating from scattering of laser light, are detected. The effect of noise photons changes the correlation function into

$$g_{\text{noise}}^{(2)}(\tau) \approx \frac{g^{(2)}(\tau) + (2 + p_n)p_n}{(1 + p_n)^2}, \quad (27)$$

where  $p_n$  is the relative rate (odds) of detecting noise photons compared to Raman photons and we have assumed that the noise photons are completely classical and uncorrelated. The results of this model are in good agreement with the measured data as shown in Fig. S10. The solid curves in Fig. 5D are a simple phenomenological model assuming exponential decay with a single timescale for the distinguishable and single-SiV cases and two timescales for the indistinguishable case. All models are convolved with the (independently measured) temporal response of the cavity and photon detectors.

### 8.3 Entanglement Analysis

We verify entanglement generation through the two-photon correlation function of the emitted field from the SiVs. The SiVs are excited by weak continuous-wave lasers and the corresponding emitted field is a stationary field such that the photon correlation function of the field can

be written as

$$g^{(2)}(\tau) = \frac{\text{Tr} \left\{ \hat{A}^\dagger \hat{A}^\dagger(\tau) \hat{A}(\tau) \hat{A} \rho \right\}}{\text{Tr} \left\{ \hat{A}^\dagger \hat{A} \rho \right\}^2} = \frac{\text{Tr} \left\{ \hat{A}^\dagger \hat{A} e^{\mathcal{L}\tau} \left[ \hat{A} \rho \hat{A}^\dagger \right] \right\}}{\text{Tr} \left\{ \hat{A}^\dagger \hat{A} \rho \right\}^2} \quad (28)$$

$$= \frac{\text{Tr} \left\{ \hat{A}^\dagger \hat{A} \tilde{\rho}(\tau) \right\}}{\text{Tr} \left\{ \hat{A}^\dagger \hat{A} \rho \right\}}, \quad (29)$$

where  $\hat{A} = \hat{A}(0)$  is the annihilation operator of the field and  $\rho$  is the density matrix describing the stationary field, i.e. the steady state density matrix of the system. We have defined  $\tilde{\rho}(\tau)$  as the conditional density matrix at time  $\tau$  with initial condition  $\tilde{\rho}(0) = \frac{1}{\text{Tr} \left\{ \hat{A}^\dagger \hat{A} \rho \right\}} \hat{A} \rho \hat{A}^\dagger$  and time evolution described by some Lindblad super-operator  $\mathcal{L}\tau$ .  $\tilde{\rho}(\tau)$  thus describes the state of the system at time  $\tau$  conditioned on having detected a photon at time  $\tau = 0$ . The photon correlation function  $g^{(2)}(\tau)$  thus directly probes the ratio between photon emission from the conditionally prepared state and the stationary state  $\rho$ .

### 8.3.1 Concurrence

The degree of entanglement of an arbitrary two qubit state can be quantified by the concurrence of the corresponding density matrix,  $\mathcal{C}(\rho)$  (15). All separable states have  $\mathcal{C}(\rho) = 0$  while a maximally entangled state has  $\mathcal{C}(\rho) = 1$ . Following the procedure of Ref. (16), we derive a lower bound on the concurrence of the state of the two SiVs conditioned on a photon detection. We show that the concurrence is positive, demonstrating the presence of entanglement after a single-photon detection.

As a general model for the SiVs, we describe them as qubits with states  $|c\rangle$  and  $|u\rangle$  where a photon can be emitted from state  $|u\rangle$  with some fixed probability while  $|c\rangle$  is dark. Let  $p_{u,i}^{(0)}$  be the probability of the  $i^{\text{th}}$  SiV to be in state  $|u\rangle$  in the steady state. According to Eq. (29), the corresponding single SiV photon correlation function can then be written as

$$g_i^{(2)}(\tau) = \frac{p_{u,i}(\tau)}{p_{u,i}^{(0)}}, \quad (30)$$

where  $p_{u,i}(\tau)$  is the probability of the SiV to be in state  $|u\rangle$  time  $\tau$  after the detection of the first photon. If both SiVs are continuously excited, we can write the density matrix following the

detection of a photon as

$$\tilde{\rho} = \begin{pmatrix} p_{cc} & 0 & 0 & 0 \\ 0 & p_{uc} & d & 0 \\ 0 & d^* & p_{cu} & 0 \\ 0 & 0 & 0 & p_{uu} \end{pmatrix}, \quad (31)$$

in the basis  $\{|cc\rangle, |cu\rangle, |uc\rangle, |uu\rangle\}$ . Here,  $p_{cu}$  is the (time-dependent) probability of the first SiV being in state  $|c\rangle$  and the second SiV being in state  $|u\rangle$ , and so on. Note that we have assumed there is no coherence in the system except between states  $|cu\rangle$  and  $|uc\rangle$ . This assumption gives a lower bound on the actual amount of entanglement in the system since any coherences could be removed with local operations on the SiVs and classical communication, which can never increase the amount of entanglement as described in Ref. (16). The concurrence of the conditional density matrix is (16)

$$\mathcal{C}(\tilde{\rho}) = \max(2|d| - 2\sqrt{p_{cc}p_{uu}}, 0). \quad (32)$$

We assume that the two SiVs are completely uncorrelated in the steady state before a photon detection and that we are detecting a mode  $\hat{A} \sim \hat{S}_1 + e^{i\phi}\hat{S}_2$ , where  $\hat{S}_i$  is the operator associated with emission of a photon from the  $i^{\text{th}}$  SiV. The  $g^{(2)}$  function can then be written as

$$g^{(2)}(\tau) = \frac{p_{cu} + p_{uc} + 2|d|\cos(\theta - \phi) + 2p_{uu}}{p_{u,1}^{(0)} + p_{u,2}^{(0)}}, \quad (33)$$

where we have written the coherences as  $d = |d|e^{i\theta}$ . From this, we obtain a lower bound on the coherences

$$2|d| \geq \left| g_{\text{indist}}^{(2)}(\tau) \left( p_{u,1}^{(0)} + p_{u,2}^{(0)} \right) - 1 - p_{uu} + p_{cc} \right|, \quad (34)$$

where we have used that  $p_{uc} + p_{cu} = 1 - p_{cc} - p_{uu}$ . The diagonal elements  $p_{uu}$  and  $p_{cc}$  can be obtained from the single-SiV  $g_i^{(2)}$  functions as

$$p_{uu} = \frac{p_{u,1}^{(0)}p_{u,2}^{(0)}}{p_{u,1}^{(0)} + p_{u,2}^{(0)}} (p_{u,1}(\tau) + p_{u,2}(\tau)) = \frac{p_{u,1}^{(0)}p_{u,2}^{(0)}}{p_{u,1}^{(0)} + p_{u,2}^{(0)}} \left( g_1^{(2)}(\tau)p_{u,1}^{(0)} + g_2^{(2)}(\tau)p_{u,2}^{(0)} \right), \quad (35)$$

and

$$p_{cc} = \frac{1}{p_{u,1}^{(0)} + p_{u,2}^{(0)}} \left( p_{c,1}(\tau)p_{c,2}^{(0)}p_{u,1}^{(0)} + p_{c,2}(\tau)p_{c,1}^{(0)}p_{u,2}^{(0)} \right) \quad (36)$$

$$= \frac{1}{p_{u,1}^{(0)} + p_{u,2}^{(0)}} \left( (1 - g_1^{(2)}(\tau)p_{u,1}^{(0)})(1 - p_{u,2}^{(0)})p_{u,1}^{(0)} + (1 - g_2^{(2)}(\tau)p_{u,2}^{(0)})(1 - p_{u,1}^{(0)})p_{u,2}^{(0)} \right), \quad (37)$$

where we have used that  $p_{c,i}^{(0)} = 1 - p_{u,i}^{(0)}$  and  $p_{c,i} = 1 - p_{u,i}$ . Combining Eqs. (34)-(36) with Eq. (32) gives a lower bound on the concurrence. For the experiment, the photon detection rates from the SiVs were balanced such that  $p_{u,1}^{(0)} = p_{u,2}^{(0)} = p_u^{(0)}$  and the lower bound becomes

$$\mathcal{C}(\tilde{\rho}) \geq \max \left( 0, \left| 2g_{\text{indist}}^{(2)}(\tau)p_u^{(0)} - \frac{1}{2} \left( 2 + g_1^{(2)}(\tau) + g_2^{(2)}(\tau) \right) p_u^{(0)} \right| - p_u^{(0)} \sqrt{\left( g_1^{(2)}(\tau) + g_2^{(2)}(\tau) \right) \left( 2 - (g_1^{(2)}(\tau) + g_2^{(2)}(\tau))p_u^{(0)} \right) (1 - p_u^{(0)})} \right). \quad (38)$$

We estimate the concurrence generated in our experiment by directly evaluating Eq. (38) using experimentally measured values of  $g^{(2)}(\tau)$  at short time delays  $\tau \sim 0$  (Fig. 5). We estimate the error assuming the photon count rates follow a Poisson distribution. (This assumption has been verified via similar measurements on the same apparatus). By taking the thermal distribution at 4 K and measured saturation associated with weak optical pumping during the measurement into account, we obtain a lower bound of  $p_u^{(0)} \geq 0.34$  for each SiV in steady state. From fits of the autocorrelation functions shown in Fig. 5D, we obtain the concurrence  $\mathcal{C}(\tau = 0) > 0.090$  (0.024) demonstrating entanglement generation in the system. Around  $\tau = 0$  the concurrence is fairly insensitive to this window size and is positive for window sizes up to 8 ns. All uncertainties given in parentheses here and throughout the manuscript are the one-standard-deviation level. Note that the extracted value of concurrence is limited by imperfect initial state preparation of the SiV centers. This can be circumvented by either working with the pulsed excitation or via post-selection as discussed in the following section.

### 8.3.2 Conditional fidelity estimate

The lower bound on the concurrence extracted above verifies that entanglement is created by the first photon. In order to relate this entanglement to the theoretical model presented previously, we now estimate the fidelity of the conditional state with state  $|B\rangle$  given that a second photon is detected at a time  $\epsilon$  after the first. Here,  $\epsilon$  is much shorter than the decoherence rate of the ground states, which ensures that any dynamics of the conditional state can be neglected and we therefore post-select on events where the initial state of the SiVs was  $|uu\rangle$  to good approximation.

While the measurement of the correlation function of a single SiV individually shows a strong anti-bunching at  $\tau = 0$  (orange curve in Fig. 5D), the correlation functions do not completely vanish as expected for an ideal single photon source. What is detected is therefore not

only the field from the Raman transition of the SiV but also noise photons originating primarily from the scattering of frequency-distinguishable laser light. From the single-emitter  $g_i^{(2)}$  functions, we can estimate the ratio,  $p_{n,i}$  between the detection rate of noise photons and Raman photons assuming that the noise photons are classical and uncorrelated. From Eq. (27), we find that

$$g_i^{(2)}(0) = \frac{p_{n,i}(2 + p_{n,i})}{(1 + p_{n,i})^2}, \quad (39)$$

which for the measured single emitter  $g^{(2)}$  functions of  $g_1^{(2)}(0) = g_2^{(2)}(0) = 0.16(3)$  gives  $p_{n,1} = p_{n,2} = p_n = 0.09(2)$ .

To calculate the  $g^{(2)}$  function when both emitters are excited, we assume that the emitters are completely uncorrelated in the steady state. Consequently, the rate of Raman photons  $\gamma_R$  is simply the sum of the Raman photon rates from the single emitters in the steady state. Furthermore, the rate of noise photons  $\gamma_{\text{noise}}$  is also assumed to be the sum of the noise photon rates for the single emitters. In the experiments, the photon detection rate from the two emitters was balanced, which means that the ratio between the detection rate of Raman photons and noise photons is still  $p_n$ . The total rate of photons from the steady state can thus be written as  $\gamma_{\text{total}} = \gamma_R + \gamma_{\text{noise}} = 2\gamma_r p_u^{(0)}(1 + p_n)$ , where we have written the single emitter Raman photon rate as  $\gamma_r p_u^{(0)}$  where  $p_u^{(0)}$  is the steady state probability of an emitter to be in state  $|u\rangle$ .

The conditional density matrix upon detection of the first photon can be parameterized as

$$\tilde{\rho} = \frac{1}{1 + p_n} \left( p_u^{(0)} \tilde{F} |B\rangle \langle B| + (1 - p_u^{(0)} \tilde{F}) \rho_d \right) + \frac{p_n}{1 + p_n} \rho, \quad (40)$$

where  $\rho$  is the steady state density matrix of the SiVs and  $\rho_d$  describes all states that cannot emit Raman photons, i.e.  $|cc\rangle$  and  $|D\rangle = \frac{1}{\sqrt{2}}(|uc\rangle - e^{i\phi}|cu\rangle)$ . The first term proportional to  $\frac{1}{1+p_n}$  can be viewed as the conditional density matrix if the first photon was a Raman photon while the second term proportional to  $\frac{p_n}{1+p_n}$  is where the first photon was a noise photon. This conditional density matrix results in a  $g^{(2)}$  function

$$g^{(2)}(0) = \frac{\tilde{F} + p_n(2 + p_n)}{(1 + p_n)^2}. \quad (41)$$

$\tilde{F}$  can thus be extracted from the measured value of  $g^{(2)}(0)$  in Fig. 5D.  $\tilde{F}$  can be viewed as the fidelity with state  $|B\rangle$  if the two SiVs were initially in state  $|uu\rangle$ .

In the  $g^{(2)}$  measurements, we postselect for experimental runs that result in a two-photon coincidence. For these runs, the overlap with state  $|B\rangle$  is then given by  $F = p_{uu}^{(c)} \tilde{F}$ , where  $p_{uu}^{(c)}$  is the probability of the initial state being  $|uu\rangle$  given that we detected the second photon  $\epsilon$  after

the first photon. This probability can be bounded from below by the relative rate of detecting two Raman photons compared to the total rate of detecting two photons. From Eq. (40), we find that this is

$$p_{uu}^{(c)} \geq \frac{\frac{1}{1+p_n} 2\tilde{F} p_u^{(0)} \gamma_s}{\frac{1}{1+p_n} 2\tilde{F} p_u^{(0)} \gamma_s + 2p_n p_u^{(0)} \gamma_s + \frac{p_n}{1+p_n} 2\gamma_s p_u^{(0)}} = \frac{\tilde{F}}{\tilde{F} + (2 + p_n)p_n}. \quad (42)$$

Consequently, we find a lower bound on the fidelity of the conditional state

$$F \geq \frac{(g^{(2)}(0)(1 + p_n)^2 - p_n(2 + p_n))^2}{g^{(2)}(0)(1 + p_n)^2}. \quad (43)$$

From the measured value of  $g^{(2)}(0) = 0.98(5)$ , we obtain  $F \geq 82(7)\%$ .

## 9 Appendix: Analytical expressions for density matrix elements

### 9.1 Steady-state density matrix expressions

The analytical expression for the matrix elements  $\rho_{i,j}^{(s)} = \langle i | \rho^{(s)} | j \rangle$  in Sec. 5.2 are given by:

$$\rho_{1,1}^{(s)} \approx \frac{1}{\mathcal{A} + \mathcal{B}/\mathcal{C}} \quad (44)$$

$$\rho_{1,2}^{(s)} \approx \frac{-4\xi g \rho_{1,1}^{(s)}}{\mathcal{C}} \times (16\xi^2 g^2 - \kappa((4\Delta_e^2 + \kappa^2)(\gamma_c + \gamma_u) + 4g^2(\kappa + \gamma_c + \gamma_u)))(4g^2 + \kappa(2i\Delta_e + \Gamma)) \quad (45)$$

$$\rho_{2,2}^{(s)} \approx \frac{16\xi^2 g^2 \kappa(\kappa + \Gamma)(4g^2 + \kappa\Gamma)\rho_{1,1}^{(s)}}{\mathcal{C}}, \quad (46)$$

$$\rho_{3,3}^{(s)} \approx \frac{\gamma_u \rho_{2,2}^{(s)} + \gamma_{uc} \rho_{1,1}^{(s)}}{\gamma_{cu}} \quad (47)$$

$$\rho_{4,4}^{(s)} \approx \frac{4\xi^2 \rho_{1,1}^{(s)}}{\mathcal{C}} \left( 16\Delta_e^4 \kappa(\gamma_c + \gamma_u) + (4g^2 + \kappa\Gamma)(16\xi^2 g^2 + \kappa(4g^2(\gamma_d + \gamma_{uc}) + \kappa(\gamma_c + \gamma_u)\Gamma)) \right. \\ \left. + 4\Delta_e^2 \kappa(\gamma_c + \gamma_u)(\kappa^2 + \Gamma^2) + 4\Delta_e^2(-16\xi^2 g^2 + 4g^2(\kappa^2 + (\kappa + \Gamma)(\gamma_c + \gamma_u))) \right) \quad (48)$$

$$\rho_{5,5}^{(s)} \approx \frac{4\xi^2}{\kappa^2} \rho_{2,2}^{(s)} \quad (49)$$

$$\rho_{6,6}^{(s)} \approx \frac{4\xi^2}{\kappa^2} \rho_{3,3}^{(s)} \quad (50)$$

$$\begin{aligned} \rho_{7,7}^{(s)} \approx & \frac{4\xi^2 \rho_{4,4}^{(s)} + 4g^2 \rho_{5,5}^{(s)}}{3\kappa^2} - \frac{8}{27\kappa^4} \left( -9\xi^4 \rho_{1,1}^{(s)} + 45\xi^3 g (\rho_{1,2}^{(s)} + \rho_{2,1}^{(s)}) \right. \\ & \left. + 12\xi^2 g^2 (-9\rho_{2,2}^{(s)} + 7\rho_{4,4}^{(s)}) + 2g^2 (\Delta_e^2 + 3g^2) \rho_{5,5}^{(s)} \right) + \frac{392i\Delta_e \xi^3 g}{9\kappa^5} (\rho_{1,2}^{(s)} - \rho_{2,1}^{(s)}) \end{aligned} \quad (51)$$

$$\rho_{8,8}^{(s)} \approx \frac{6\xi^2}{3\kappa^2} \rho_{6,6}^{(s)}, \quad (52)$$

where we have defined

$$\mathcal{A} = \frac{\gamma_{cu} + \gamma_{uc}}{\gamma_{cu}} + \left( \frac{8\xi^4 + 4\xi^2 \kappa^2}{\kappa^4} \right) \frac{\gamma_{uc}}{\gamma_{cu}} \quad (53)$$

$$\begin{aligned} \mathcal{B} = & \frac{16g^2 \xi^2}{3\kappa^3 \gamma_{cu}} (24\xi^4 \gamma_u + 3\kappa^4 (\gamma_{cu} + \gamma_u) + 4\xi^2 (4g^2 \gamma_{cu} + 3\kappa^2 (\gamma_{cu} + \gamma_u))) (\kappa + \Gamma) (4g^2 + \kappa \Gamma) \\ & + \left( 4\xi^2 + \frac{16\xi^4}{3\kappa^2} \right) \left( 16\Delta_e^4 \kappa (\gamma_c + \gamma_u) + (4g^2 + \kappa \Gamma) (16\xi^2 g^2 + \kappa (4g^2 (\gamma_d + \gamma_{uc}) + \kappa (\gamma_c + \gamma_u) \Gamma)) \right. \\ & \left. + 4\Delta_e^2 (-16\xi^2 g^2 + 4g^2 (\kappa^2 + (\kappa + \Gamma) (\gamma_c + \gamma_u)) + \kappa (\gamma_u + \gamma_c) (\kappa^2 + \Gamma^2)) \right) \end{aligned} \quad (54)$$

$$\begin{aligned} \mathcal{C} = & -16\xi^2 g^2 (4\Delta_e^2 \kappa^2 + (4g^2 - \kappa^2) (4g^2 + \kappa \Gamma)) \\ & + \kappa ((4\Delta_e^2 + \kappa^2) (\gamma_c + \gamma_u) + 4g^2 (\kappa + \gamma_c + \gamma_u)) (4\Delta_e^2 \kappa^2 + (4g^2 + \kappa \Gamma)^2). \end{aligned} \quad (55)$$

## 9.2 Coefficients in the expressions for the time-dependent density matrix elements

Here, we give explicit expressions for the coefficients  $a_i$ ,  $b_i$ ,  $\mathcal{A}_i$ ,  $\mathcal{B}_i$  and  $\mathcal{C}_i$  in the time-dependent density matrix elements described in Sec. 5.3:

$$\mathcal{A}_1 = -\frac{a_2}{a_1 + i\Delta_e}, \quad \mathcal{C}_1 = \frac{1}{\kappa^2 + 4g^2} (4\xi^2\alpha - 4\xi g (\mathcal{A}_1 + \mathcal{A}_1^*) + 4g^2\mathcal{B}_1), \quad (56)$$

$$\mathcal{A}_2 = -\frac{a_3}{a_1 + i\Delta_e + \tilde{\gamma}}, \quad \mathcal{C}_2 = \frac{1}{\kappa^2 + 4g^2} (4\xi^2\beta - 4\xi g (\mathcal{A}_2 + \mathcal{A}_2^*) + 4g^2\mathcal{B}_2), \quad (57)$$

$$\mathcal{A}_3 = (-\mathcal{A}_1 - \mathcal{A}_2 + \rho_{1,2}(0)) e^{i\Delta_e t}, \quad \mathcal{C}_3 = \frac{1}{\kappa^2 + 4g^2} (-4\xi g (\mathcal{A}_3 + \mathcal{A}_3^*) + 4g^2\mathcal{B}_3), \quad (58)$$

$$\mathcal{B}_1 = \frac{2a_1a_2b_2}{b_1(a_1^2 + \Delta_e^2)} - \frac{b_3}{b_1}, \quad \mathcal{C}_4 = \frac{4g^2}{\kappa^2 + 4g^2}\mathcal{B}_4, \quad (59)$$

$$\begin{aligned} \mathcal{B}_2 = & \frac{-(a_1^2 + \Delta_e^2)b_4 + a_1a_3b_2}{(b_1 + \tilde{\gamma})(\Delta_e^2 + (a_1 + \tilde{\gamma})^2)} \\ & - \frac{(b_4(2a_1 + \tilde{\gamma}) - 2a_3b_2)(\tilde{\gamma})}{(b_1 + \tilde{\gamma})(\Delta_e^2 + (a_1 + \tilde{\gamma})^2)}, \quad \mathcal{B}_4 = -(\mathcal{B}_1 + \mathcal{B}_2) + \rho_{2,2}(0) \\ & - 2\Re \left[ \frac{b_2}{a_1 + i\Delta_e - b_1} \mathcal{A}_3 e^{-i\Delta_e t} \right], \end{aligned} \quad (60)$$

$$\mathcal{B}_3 = 2\Re \left[ \frac{b_2}{a_1 + i\Delta_e - b_1} \mathcal{A}_3 \right], \quad (61)$$

and

$$b_1 = -\gamma_c - \gamma_u - \frac{4g^2\kappa}{\kappa^2 + 4g^2}, \quad a_1 = -\frac{\gamma_u + \gamma_c + \gamma_d + \gamma_{uc}}{2} - \frac{2g^2}{\kappa}, \quad (62)$$

$$b_2 = \frac{2\xi g}{\kappa} - \frac{16g^3\xi}{\kappa(\kappa^2 + 4g^2)}, \quad a_2 = \frac{2g\xi}{\kappa}\alpha, \quad (63)$$

$$b_3 = \frac{16\xi^2g^2}{\kappa(\kappa^2 + 4g^2)}\alpha, \quad a_3 = \frac{2g\xi}{\kappa}\beta, \quad (64)$$

$$b_4 = \frac{16\xi^2g^2}{\kappa(\kappa^2 + 4g^2)}\beta. \quad (65)$$

### 9.3 Coefficients and matrix elements for the two-SiV model

The constants and matrix elements appearing in Sec. 8.2 are defined as

$$\alpha_1 = \frac{4|g_1|^2|\Omega_1|^2}{\Delta_1^2\kappa^2}, \quad \alpha_2 = \frac{4|g_2|^2|\Omega_2|^2}{\Delta_2^2\kappa^2}, \quad (66)$$

$$\alpha_3 = \frac{4g_1^*g_2\Omega_2^*\Omega_1}{\Delta_1\Delta_2\kappa^2}, \quad \rho_{1,1}^{(s)} \approx \frac{\gamma_{uc}^2}{(\gamma_{uc} + \gamma_{cu})^2} \quad (67)$$

$$\rho_{2,2}^{(s)} \approx \frac{\gamma_{uc}\gamma_{cu}}{(\gamma_{uc} + \gamma_{cu})^2}, \quad \rho_{4,4}^{(s)} \approx \frac{\gamma_{cu}^2}{(\gamma_{uc} + \gamma_{cu})^2} \quad (68)$$

$$\rho_{1,1}(\tau) \approx \beta_1 (1 - e^{-\tilde{\gamma}\tau}), \quad \rho_{2,2}(\tau) \approx \beta_2 + e^{-\tilde{\gamma}\tau}\beta_3 \quad (69)$$

$$\rho_{3,3}(\tau) \approx \beta_2 + e^{-\tilde{\gamma}\tau}\beta_4, \quad \rho_{2,3}(\tau) \approx \alpha_3^*\rho_{1,1}^{(s)}e^{-\Gamma\tau}, \quad (70)$$

where

$$\tilde{\gamma} = \gamma_{cu} + \gamma_{uc}, \quad (71)$$

$$\Gamma = \tilde{\gamma} + \gamma_d \quad (72)$$

$$\beta_1 = (\alpha_1 + \alpha_2)(\rho_{1,1}^{(s)} + \rho_{2,2}^{(s)})\rho_{1,1}^{(s)}, \quad (73)$$

$$\beta_2 = (\alpha_1 + \alpha_2)(\rho_{1,1}^{(s)} + \rho_{2,2}^{(s)})\rho_{2,2}^{(s)}, \quad (74)$$

$$\beta_3 = -\alpha_1\rho_{2,2}^{(s)}(\rho_{1,1}^{(s)} + \rho_{2,2}^{(s)}) + \alpha_2 \left( \left( \rho_{1,1}^{(s)} \right)^2 - \left( \rho_{2,2}^{(s)} \right)^2 + \rho_{1,1}^{(s)} \left( \rho_{2,2}^{(s)} + \rho_{4,4}^{(s)} \right) \right), \quad (75)$$

$$\beta_4 = -\alpha_2\rho_{2,2}^{(s)}(\rho_{1,1}^{(s)} + \rho_{2,2}^{(s)}) + \alpha_1 \left( \left( \rho_{1,1}^{(s)} \right)^2 - \left( \rho_{2,2}^{(s)} \right)^2 + \rho_{1,1}^{(s)} \left( \rho_{2,2}^{(s)} + \rho_{4,4}^{(s)} \right) \right). \quad (76)$$

## References

1. Q. Quan, M. Lončar, *Opt. Express* **19**, 18529 (2011).
2. H. A. Atikian, *et al.*, *Appl. Phys. Lett.* **104**, 122602 (2014).
3. M. J. Burek, *et al.*, *Nano Lett.* **12**, 6084 (2012).
4. M. J. Burek, *et al.*, *Nat. Commun.* **5**, 5718 (2014).
5. Y. Chu, *et al.*, *Nano Lett.* **14**, 1982 (2014).
6. R. E. Evans, A. Sipahigil, D. D. Sukachev, A. S. Zibrov, M. D. Lukin, *Phys. Rev. Appl.* **5**, 044010 (2016).
7. S. Mosor, *et al.*, *Appl. Phys. Lett.* **87**, (2005).
8. J. F. Ziegler, M. D. Ziegler, J. P. Biersack, *Nucl. Instrum. Meth. B* **268**, 1818 (2010).
9. U. F. S. D’Haenens-Johansson, *et al.*, *Phys. Rev. B* **84**, 245208 (2011).
10. T. Tiecke, *et al.*, *Optica* **2**, 70 (2015).
11. C. Hepp, *et al.*, *Phys. Rev. Lett.* **112**, 036405 (2014).
12. H. Sternschulte, K. Thonke, R. Sauer, P. C. Münzinger, P. Michler, *Phys. Rev. B* **50**, 14554 (1994).
13. K. D. Jahnke, *et al.*, *New J. Phys.* **17**, 043011 (2015).
14. L. J. Rogers, *et al.*, *Phys. Rev. B* **89**, 235101 (2014).
15. W. K. Wootters, *Phys. Rev. Lett.* **80**, 2245 (1998).
16. C. W. Chou, *et al.*, *Nature* **438**, 828 (2005).
